# Supplementary material for: Rethinking Link Prediction for Directed Graphs
Source: arXiv:2502.05724 source file (2025-05-21)
Supplement: Supplementary file 1 [file appendix_allresults.tex]

\clearpage
\hypertarget{app_complete_res}{}
\section{Complete Results of DirLinkBench on Seven Datasets}\label{app_complete_res}

\hypertarget{app_complete_res_cora}{}
\subsection{Results on Cora-ML}\label{app_complete_res_cora}
%Table~\ref{app_tb_cora_ml} shows the results of DirLinkBench on Cora-ML.
\begin{table}[h]
    \centering
    \caption{Benchmark Results on Cora-ML. For all methods, $_{\text{F}}$ indicates the use of original node features as input, while $_{\text{D}}$ indicates the use of in/out degrees as input. Results ranked \hig{1}{first} and \hig{2}{second} are highlighted.}
    \label{app_tb_cora_ml}
    \resizebox{\textwidth}{!}{
    \begin{tabular}{lccccccc}
        \toprule
        Method & Hits@20 & Hits@50 & Hits@100 & MRR & AUC & AP & ACC \\
        \midrule
        STRAP & 67.10$\pm$2.55 & 75.05$\pm$1.66 & 79.09$\pm$1.57 & \hig{1}{30.91$\pm$7.48} & 87.38$\pm$0.83 & 90.46$\pm$0.70 & 78.47$\pm$0.77 \\
        
        ODIN & 27.10$\pm$3.69 & 40.99$\pm$3.10 & 54.85$\pm$2.53 & 10.75$\pm$3.51 & 85.15$\pm$0.84 & 85.41$\pm$0.95 & 77.16$\pm$0.84  \\
        
        ELTRA &\hig{2}{70.74$\pm$5.47} & \hig{2}{81.93$\pm$2.38} & \hig{2}{87.45$\pm$1.48} & 19.77$\pm$5.22 & 94.83$\pm$0.58 & 95.37$\pm$0.52 & 85.40$\pm$0.45  \\ \midrule
        
        MLP$_{\text{F}}$ & 27.16$\pm$6.70 & 44.28$\pm$5.72 & 60.61$\pm$6.64 & 9.02$\pm$3.58 & 89.93$\pm$2.09 & 88.55$\pm$2.51 & 81.32$\pm$2.41 \\ 
        MLP$_{\text{D}}$ & 29.84$\pm$4.83 & 44.11$\pm$4.73 & 56.74$\pm$2.03 & 11.84$\pm$3.40 & 86.44$\pm$0.74 & 86.58$\pm$0.88 & 77.95$\pm$0.95 \\ \midrule
        
        GCN$_{\text{F}}$ & 37.88$\pm$5.60 & 55.31$\pm$4.46 & 70.15$\pm$3.01 & 14.25$\pm$3.49 & 92.01$\pm$1.64 & 91.45$\pm$1.47 & 82.82$\pm$0.86 \\
        GCN$_{\text{D}}$& 31.36$\pm$3.89 & 45.03$\pm$2.92 & 58.77$\pm$2.96 & 12.56$\pm$2.86 & 86.12$\pm$0.87 & 86.79$\pm$1.01 & 77.81$\pm$0.87   \\ \midrule
        
        GAT$_{\text{F}}$ & 33.42$\pm$8.93 & 58.40$\pm$6.55 & 79.72$\pm$3.07 & 9.30$\pm$3.39 & 94.57$\pm$0.45 & 92.77$\pm$0.42 & 88.95$\pm$0.71  \\
        GAT$_{\text{D}}$ & 30.19$\pm$4.23 & 43.53$\pm$2.93 & 55.09$\pm$3.34 & 11.07$\pm$3.68 & 85.52$\pm$1.27 & 86.19$\pm$0.96 & 77.36$\pm$1.13 \\ \midrule
        
        APPNP$_{\text{F}}$ & 55.47$\pm$4.63 & 75.16$\pm$4.09 & 86.02$\pm$2.88 & 22.49$\pm$6.33 & 95.94$\pm$0.57 & \hig{2}{95.82$\pm$0.59} &\hig{2}{89.90$\pm$0.73} \\ 
        APPNP$_{\text{D}}$ & 32.21$\pm$3.65 & 45.51$\pm$3.76 & 60.02$\pm$3.36 & 11.89$\pm$2.65 & 88.00$\pm$1.08 & 88.01$\pm$1.17 & 79.28$\pm$1.13 \\\midrule
        
        DGCN$_{\text{F}}$ & 30.86$\pm$4.17 & 41.82$\pm$4.43 & 54.38$\pm$4.97 & 11.01$\pm$4.23 & 85.55$\pm$3.40 & 85.66$\pm$2.35 & 77.82$\pm$3.49  \\
        DGCN$_\text{D}$ & 36.30$\pm$4.43 & 50.25$\pm$3.42 & 63.32$\pm$2.59 & 13.98$\pm$4.24 & 87.87$\pm$0.96 & 88.67$\pm$0.84 & 80.26$\pm$0.69 \\ \midrule
        
        DiGCN$_{\text{F}}$ & 30.05$\pm$5.45 & 48.87$\pm$5.25 & 63.21$\pm$5.72 & 10.16$\pm$4.25 & 89.48$\pm$1.83 & 89.10$\pm$1.99 & 82.47$\pm$0.97 \\
        DiGCN$_{\text{D}}$ & 34.39$\pm$3.69 & 49.66$\pm$4.14 & 60.10$\pm$4.04 & 12.49$\pm$3.83 & 85.87$\pm$1.22 & 87.13$\pm$1.18 & 77.88$\pm$1.01 \\ \midrule
        
        DiGCNIB$_{\text{F}}$& 45.90$\pm$4.97 & 66.62$\pm$3.67 & 80.57$\pm$3.21 & 17.08$\pm$3.90 & 94.67$\pm$0.56 & 94.21$\pm$0.65 & 87.25$\pm$0.58 \\

        DiGCNIB$_{\text{D}}$ & 37.18$\pm$4.60 & 51.64$\pm$3.69 & 64.72$\pm$3.43 & 12.71$\pm$4.08 & 89.23$\pm$0.92 & 89.36$\pm$0.85 & 81.05$\pm$1.05 \\ \midrule
        
        DirGNN$_{\text{F}}$ & 42.48$\pm$7.34 & 59.41$\pm$4.00 & 76.13$\pm$2.85 & 12.01$\pm$3.57 & 93.05$\pm$0.87 & 92.52$\pm$0.79 & 85.83$\pm$0.93 \\
        DirGNN$_{\text{D}}$ & 32.29$\pm$2.25 & 45.53$\pm$2.60 & 58.22$\pm$2.50 & 13.34$\pm$5.56 &87.06$\pm$ 0.77 &87.35$\pm$0.80 & 77.93$\pm$1.14 \\ \midrule
        
        MagNet$_{\text{F}}$ & 26.87$\pm$3.82 & 40.58$\pm$3.19 & 53.51$\pm$2.00 & 10.08$\pm$3.47 & 85.21$\pm$0.79 & 85.53$\pm$1.00 & 76.93$\pm$0.79 \\
        MagNet$_{\text{D}}$ & 29.38$\pm$3.39 & 43.28$\pm$3.76 & 56.54$\pm$2.95 & 11.19$\pm$3.04 & 85.23$\pm$0.84 & 86.06$\pm$0.94 & 77.51$\pm$0.92 \\ \midrule

        DUPLEX$_{\text{F}}$ & 21.73$\pm$3.19 & 34.98$\pm$2.37 & 69.00$\pm$2.52 & 7.74$\pm$1.95 & 88.02$\pm$0.95 & 86.62$\pm$1.43 & 82.28$\pm$0.93 \\
        DUPLEX$_{\text{D}}$& 17.48$\pm$4.69 & 32.58$\pm$8.33 & 54.50$\pm$7.49 & 5.46$\pm$2.10 & 82.97$\pm$4.47 & 82.97$\pm$2.85 & 75.59$\pm$4.87 \\ \midrule

        DHYPR$_{\text{F}}$ & 59.81$\pm$4.79 & 77.45$\pm$2.56 & 86.81$\pm$1.60 & 20.56$\pm$5.10 & \hig{2}{96.13$\pm$0.28} & 95.84$\pm$0.39 & 86.04$\pm$0.66  \\
        DHYPR$_{\text{D}}$ & 15.09$\pm$4.40 & 28.96$\pm$6.54 & 42.93$\pm$6.63 & 4.05$\pm$1.16 & 80.83$\pm$2.64 & 79.97$\pm$3.02 & 72.74$\pm$3.50 \\ \midrule
        
        DiGAE$_{\text{F}}$& 56.13$\pm$3.80 & 72.23$\pm$2.51 & 82.06$\pm$2.51 & 20.53$\pm$4.21 & 92.56$\pm$0.66 & 93.70$\pm$0.54 & 86.25$\pm$0.80  \\
        DiGAE$_{\text{D}}$ & 35.40$\pm$4.05 & 49.12$\pm$3.44 & 61.30$\pm$2.70 & 13.71$\pm$4.22 & 86.82$\pm$0.85 & 87.35$\pm$0.84 & 76.01$\pm$1.04 \\ \midrule

        %SDGAE$_{\text{F}}$ &\textbf{70.89$\pm$3.35} & \textbf{83.63$\pm$2.15} & \textbf{90.37$\pm$1.33} & \underline{28.45$\pm$5.82} & \textbf{97.24$\pm$0.34} & \textbf{97.21$\pm$0.17} & \textbf{91.36$\pm$0.70}  \\ 
        SDGAE$_{\text{F}}$ &\hig{1}{70.89$\pm$3.35} & \hig{1}{83.63$\pm$2.15} &\hig{1}{90.37$\pm$1.33} & \hig{2}{28.45$\pm$5.82} & \hig{1}{97.24$\pm$0.34} & \hig{1}{97.21$\pm$0.17} &\hig{1}{91.36$\pm$0.70}  \\

        SDGAE$_{\text{D}}$& 35.53$\pm$5.41 & 49.34$\pm$4.60 & 61.40$\pm$3.18 & 14.21$\pm$3.71 & 87.38$\pm$1.06 & 88.19$\pm$1.18 & 78.99$\pm$1.34  \\

        \bottomrule
    \end{tabular}}
\end{table}

\clearpage
\hypertarget{app_complete_res_citeseer}{}
\subsection{Results on CiteSeer}\label{app_complete_res_citeseer}
%Table~\ref{app_tb_citeseer} shows the results of DirLinkBench on CiteSeer.
\begin{table}[h]
    \centering
    \caption{Benchmark Results on CiteSeer. For all methods, $_{\text{F}}$ indicates the use of original node features as input, while $_{\text{D}}$ indicates the use of in/out degrees as input. Results ranked \hig{1}{first} and \hig{2}{second} are highlighted.}
    \label{app_tb_citeseer}
    \resizebox{\textwidth}{!}{
    \begin{tabular}{lccccccc}
        \toprule
        Model & Hits@20 & Hits@50 & Hits@100 & MRR & AUC & AP & ACC \\
        \midrule
        STRAP & 63.28$\pm$1.46 & 67.05$\pm$1.32 & 69.32$\pm$1.29 & \hig{2}{40.70$\pm$6.95} & 81.82$\pm$1.44 & 84.15$\pm$0.84 & 75.01$\pm$1.40 \\
        
        ODIN & 30.74$\pm$3.78 & 47.91$\pm$2.57 & 63.95$\pm$2.98 & 11.05$\pm$2.74 & 82.22$\pm$1.05 & 81.74$\pm$1.10 & 73.63$\pm$1.19  \\
        
        ELTRA & 72.34$\pm$1.76 & 79.44$\pm$1.54 & 84.97$\pm$1.90 & 27.87$\pm$9.03 & 90.98$\pm$0.86 & 92.71$\pm$0.81 & 80.86$\pm$1.15  \\ \midrule
        
        MLP$_{\text{F}}$& 35.55$\pm$4.39 & 52.31$\pm$4.60 & 70.27$\pm$3.40 & 16.08$\pm$4.88 & 85.47$\pm$1.35 & 85.16$\pm$1.29 & 74.26$\pm$1.64  \\
        MLP$_{\text{D}}$ & 40.27$\pm$4.48 & 56.27$\pm$3.64 & 68.78$\pm$2.21 & 15.94$\pm$3.04 & 84.09$\pm$1.02 & 84.86$\pm$1.12 & 74.81$\pm$1.32  \\ \midrule
        
        GCN$_{\text{F}}$ & 42.27$\pm$7.11 & 62.65$\pm$4.22 & 80.36$\pm$3.07 & 18.28$\pm$6.7 & 89.94$\pm$1.04 & 88.88$\pm$1.38 & 79.47$\pm$1.73 \\
        GCN$_{\text{D}}$ & 43.96$\pm$2.35 & 56.24$\pm$3.62 & 66.15$\pm$2.07 & 19.36$\pm$4.96 & 81.24$\pm$1.55 & 84.33$\pm$0.90 & 73.92$\pm$1.43 \\ \midrule

        GAT$_{\text{F}}$ & 48.29$\pm$6.04 & 71.86$\pm$4.65 & 85.88$\pm$4.98 & 16.71$\pm$5.56 & 92.90$\pm$0.74 & 91.12$\pm$1.53 & 85.94$\pm$1.21 \\
        GAT$_{\text{D}}$ & 40.29$\pm$3.25 & 55.62$\pm$1.92 & 65.82$\pm$2.87 & 19.00$\pm$4.18 & 82.72$\pm$0.67 & 83.96$\pm$0.60 & 74.18$\pm$1.18 \\ \midrule

        APPNP$_{\text{F}}$& 59.86$\pm$6.54 & 77.57$\pm$5.68 & 83.57$\pm$4.90 & 20.91$\pm$4.39 & 93.58$\pm$0.71 & 93.09$\pm$0.68 & 86.23$\pm$1.49  \\
        APPNP$_{\text{D}}$ & 45.44$\pm$3.38 & 58.18$\pm$1.55 & 68.47$\pm$3.00 & 20.18$\pm$5.50 & 83.48$\pm$1.17 & 85.72$\pm$1.00 & 74.86$\pm$1.19 \\ \midrule

        DGCN$_{\text{F}}$ & 39.64$\pm$6.53 & 50.85$\pm$2.91 & 62.97$\pm$4.79 & 19.15$\pm$4.34 & 80.60$\pm$2.90 & 81.80$\pm$1.85 & 74.12$\pm$2.49  \\
        DGCN$_{\text{D}}$ & 45.94$\pm$3.01 & 58.38$\pm$2.85 & 68.97$\pm$3.39 & 19.53$\pm$4.83 & 83.38$\pm$1.41 & 85.44$\pm$1.01 & 74.83$\pm$1.46  \\ \midrule

        DiGCN$_{\text{F}}$ & 38.48$\pm$3.50 & 53.30$\pm$5.92 & 70.95$\pm$4.67 & 15.79$\pm$4.05 & 87.41$\pm$2.24 & 85.02$\pm$2.90 & 80.38$\pm$1.17 \\
        DiGCN$_{\text{D}}$ & 40.65$\pm$4.23 & 52.87$\pm$3.85 & 65.46$\pm$3.70 & 17.39$\pm$4.82 & 83.50$\pm$1.12 & 84.75$\pm$0.93 & 74.65$\pm$1.36  \\ \midrule

        DiGCNIB$_{\text{F}}$& 44.90$\pm$7.91 & 69.86$\pm$5.13 & 85.32$\pm$3.70 & 16.61$\pm$5.61 & 92.50$\pm$0.57 & 90.35$\pm$1.43 & 85.98$\pm$1.19 \\
        DiGCNIB$_{\text{D}}$ & 45.68$\pm$3.50 & 58.99$\pm$3.92 & 70.29$\pm$2.39 & 20.22$\pm$3.31 & 85.81$\pm$0.69 & 86.73$\pm$0.85 & 76.54$\pm$1.27 \\ \midrule

        DirGNN$_{\text{F}}$ & 44.95$\pm$7.31 & 64.00$\pm$3.19 & 76.83$\pm$4.24 & 16.19$\pm$4.51 & 88.44$\pm$1.28 & 88.59$\pm$1.14 & 80.34$\pm$1.52 \\
        DirGNN$_{\text{D}}$ & 40.16$\pm$4.84 & 53.44$\pm$3.38 & 65.62$\pm$2.46 & 16.95$\pm$5.45 & 83.67$\pm$1.08 & 84.59$\pm$1.18 & 73.75$\pm$1.31 \\ \midrule
        
        MagNet$_{\text{F}}$ & 32.18$\pm$5.04 & 47.44$\pm$3.24 & 61.55$\pm$8.45 & 12.97$\pm$1.73 & 82.58$\pm$1.31 & 82.70$\pm$1.45 & 73.73$\pm$1.30 \\
        MagNet$_{\text{D}}$ & 39.35$\pm$5.13 & 54.50$\pm$3.21 & 65.32$\pm$3.26 & 15.31$\pm$2.45 & 83.05$\pm$1.35 & 84.14$\pm$1.31 & 73.28$\pm$1.21  \\ \midrule

        DUPLEX$_{\text{F}}$ & 30.16$\pm$5.06 & 50.90$\pm$10.69 & 73.39$\pm$3.42 & 17.82$\pm$4.47 & 84.63$\pm$2.20 & 83.01$\pm$2.10 & 79.20$\pm$1.79 \\ 
        DUPLEX$_{\text{D}}$ &27.98$\pm$7.61 & 50.20$\pm$7.36 & 63.62$\pm$3.90 & 10.95$\pm$6.35 & 80.68$\pm$1.15 & 81.17$\pm$1.20 & 73.75$\pm$1.44 \\ \midrule

        DHYPR$_{\text{F}}$ &\hig{2}{77.77$\pm$4.10} & \hig{2}{89.35$\pm$2.59} & \hig{2}{92.32$\pm$3.72} & 32.39$\pm$10.14 & \hig{2}{96.61$\pm$0.28} & \hig{2}{96.35$\pm$0.50} & \hig{2}{87.33$\pm$1.39}  \\
        DHYPR$_{\text{D}}$ & 24.32$\pm$8.59 & 41.51$\pm$6.55 & 54.27$\pm$5.94 & 6.17$\pm$2.12 & 77.38$\pm$1.79 & 77.35$\pm$2.44 & 70.27$\pm$1.35 \\  \midrule
        
        DiGAE$_{\text{F}}$ & 56.12$\pm$3.08 & 71.06$\pm$2.49 & 83.64$\pm$3.21 & 22.88$\pm$6.79 & 91.03$\pm$1.14 & 91.29$\pm$1.04 & 81.85$\pm$1.31  \\
        DiGAE$_{\text{D}}$ &  44.32$\pm$1.85 & 59.91$\pm$2.08 & 69.66$\pm$2.11 & 20.89$\pm$4.81 & 85.28$\pm$0.96 & 86.28$\pm$0.96 & 74.54$\pm$0.91 \\ \midrule

        SDGAE$_{\text{F}}$ &\hig{1}{81.06$\pm$4.50} & \hig{1}{91.24$\pm$2.55} &\hig{1}{93.69$\pm$3.68} &\hig{1}{42.50$\pm$9.76} & \hig{1}{97.24$\pm$0.60} & \hig{1}{97.13$\pm$0.68} & \hig{1}{91.38$\pm$0.79} \\ 
        SDGAE$_{\text{D}}$ & 45.03$\pm$3.19 & 57.82$\pm$2.00 & 68.97$\pm$1.70 & 21.41$\pm$2.85 & 85.10$\pm$0.98 & 86.24$\pm$0.47 & 74.83$\pm$0.86 \\

        \bottomrule
    \end{tabular}}
\end{table}

\clearpage
\hypertarget{app_complete_res_photo}{}
\subsection{Results on Photo}\label{app_complete_res_photo}
%Table~\ref{app_tb_photo} shows the results of DirLinkBench on Photo.
\begin{table}[h]
    \centering
    \caption{Benchmark Results on Photo. For all methods, $_{\text{F}}$ indicates the use of original node features as input, while $_{\text{D}}$ indicates the use of in/out degrees as input. Results ranked \hig{1}{first} and \hig{2}{second} are highlighted.}
    \label{app_tb_photo}
    \resizebox{\textwidth}{!}{
    \begin{tabular}{lccccccc}
        \toprule
        Model & Hits@20 & Hits@50 & Hits@100 & MRR & AUC & AP & ACC \\
        \midrule
        STRAP & \hig{2}{38.54$\pm$5.20} & \hig{2}{55.21$\pm$2.19} & \hig{1}{69.16$\pm$1.44} & 12.08$\pm$3.15 & 98.54$\pm$0.04 & 98.65$\pm$0.05 & 94.61$\pm$0.10 \\
        
        ODIN & 5.28$\pm$1.36 & 9.38$\pm$1.54 & 14.13$\pm$1.92 & 1.78$\pm$0.66 & 88.15$\pm$0.21 & 87.34$\pm$0.30 & 80.60$\pm$0.20  \\
        
        ELTRA & 7.09$\pm$1.23 & 12.86$\pm$1.58 & 20.63$\pm$1.93 & 2.22$\pm$0.59 & 96.89$\pm$0.06 & 95.84$\pm$0.13 & 91.84$\pm$0.12 \\ \midrule
        
        MLP$_{\text{F}}$ & 8.83$\pm$2.06 & 14.07$\pm$2.87 & 20.91$\pm$4.18 & 3.18$\pm$1.06 & 95.29$\pm$0.37 & 93.60$\pm$1.06 & 88.31$\pm$0.50  \\
        MLP$_{\text{D}}$ & 7.88$\pm$1.56 & 12.90$\pm$0.81 & 18.04$\pm$1.35 & 2.53$\pm$0.40 & 85.90$\pm$0.44 & 86.44$\pm$0.21 & 77.25$\pm$0.51  \\ \midrule
        
        GCN$_{\text{F}}$ & 29.44$\pm$3.90 & 44.12$\pm$3.49 & 57.55$\pm$2.54 & 9.85$\pm$2.78 & 99.04$\pm$0.06 & 98.66$\pm$0.10 & 95.90$\pm$0.18  \\
        GCN$_{\text{D}}$ & 31.47$\pm$3.71 & 44.93$\pm$3.34 & 58.77$\pm$2.96 & \hig{2}{12.56$\pm$2.86} & 86.12$\pm$0.87 & 86.79$\pm$1.01 & 77.71$\pm$1.01  \\ \midrule
        
        GAT$_{\text{F}}$ & 25.97$\pm$4.22 & 42.85$\pm$4.90 & 58.06$\pm$4.03 & 8.62$\pm$3.07 & \hig{2}{99.13$\pm$0.09} & \hig{2}{98.93$\pm$0.11} & \hig{1}{96.17$\pm$0.20} \\
        GAT$_{\text{D}}$ & 11.96$\pm$1.60 & 21.83$\pm$2.98 & 31.51$\pm$2.16 & 3.61$\pm$0.94 & 94.41$\pm$0.19 & 94.37$\pm$0.19 & 87.00$\pm$0.25 \\ \midrule

        APPNP$_{\text{F}}$ & 22.13$\pm$2.60 & 35.30$\pm$2.04 & 47.51$\pm$2.51 & 6.56$\pm$1.14 & 98.54$\pm$0.09 & 98.26$\pm$0.12 & 94.71$\pm$0.29 \\ 
        APPNP$_{\text{D}}$& 12.92$\pm$1.06 & 19.42$\pm$2.24 & 26.66$\pm$2.14 & 4.63$\pm$1.10 & 93.29$\pm$0.42 & 92.86$\pm$0.40 & 85.36$\pm$0.39  \\ \midrule
        
        DGCN$_{\text{F}}$ & 22.61$\pm$4.58 & 37.09$\pm$5.38 & 51.61$\pm$6.33 & 6.38$\pm$1.49 & 98.74$\pm$0.39 & 98.49$\pm$0.45 & 95.27$\pm$0.94 \\
        DGCN$_{\text{D}}$ & 15.96$\pm$3.35 & 26.88$\pm$2.91 & 35.56$\pm$3.52 & 5.83$\pm$1.16 & 96.26$\pm$0.70 & 95.94$\pm$0.76 & 90.02$\pm$1.00 \\ \midrule

        DiGCN$_{\text{F}}$ & 18.47$\pm$1.89 & 29.63$\pm$2.28 & 40.17$\pm$2.38 & 6.41$\pm$2.41 & 98.10$\pm$0.10 & 97.69$\pm$0.14 & 93.86$\pm$0.23 \\
        DiGCN$_{\text{D}}$ & 17.00$\pm$1.84 & 25.51$\pm$1.39 & 33.73$\pm$1.95 & 5.71$\pm$1.32 & 95.21$\pm$0.19 & 95.09$\pm$0.21 & 88.29$\pm$0.26 \\ \midrule
        
        DiGCNIB$_{\text{F}}$ & 21.42$\pm$2.77 & 34.97$\pm$2.67 & 48.26$\pm$3.98 & 6.82$\pm$1.53 & 98.67$\pm$0.14 & 98.39$\pm$0.16 & 95.05$\pm$0.27 \\
        DiGCNIB$_{\text{D}}$ & 16.00$\pm$1.67 & 24.63$\pm$1.84 & 33.20$\pm$2.17 & 6.11$\pm$1.50 & 96.71$\pm$0.07 & 96.38$\pm$0.09 & 91.30$\pm$0.17 \\ \midrule
        
        DirGNN$_{\text{F}}$& 22.59$\pm$2.77 & 34.65$\pm$3.31 & 49.15$\pm$3.62 & 8.42$\pm$2.90 & 98.76$\pm$0.09 & 98.47$\pm$0.13 & 95.34$\pm$0.17 \\
        DirGNN$_{\text{D}}$ &21.57$\pm$2.11 & 30.87$\pm$2.35 & 43.21$\pm$2.19 & 8.72$\pm$2.08 & 97.53$\pm$0.09 & 97.26$\pm$0.08 & 92.41$\pm$0.20 \\ \midrule
        
        MagNet$_{\text{F}}$ & 5.35$\pm$0.50 & 8.52$\pm$0.85 & 12.66$\pm$1.03 & 1.62$\pm$0.39 & 87.92$\pm$0.22 & 87.19$\pm$0.32 & 80.16$\pm$0.23 \\
        MagNet$_{\text{D}}$ & 5.14$\pm$0.54 & 9.04$\pm$0.52 & 13.89$\pm$0.32 & 1.61$\pm$0.31 & 88.11$\pm$0.21 & 87.48$\pm$0.21 & 80.31$\pm$0.14 \\ \midrule
        
        DUPLEX$_{\text{F}}$ & 7.84$\pm$1.17 & 12.64$\pm$1.22 & 17.94$\pm$0.66 & 2.53$\pm$0.66 & 94.22$\pm$0.76 & 93.37$\pm$0.91 & 87.68$\pm$0.52 \\ 
        DUPLEX$_{\text{D}}$ & 6.97$\pm$2.14 & 9.08$\pm$4.95 & 13.28$\pm$6.14 & 2.26$\pm$1.17 & 87.41$\pm$7.05 & 86.40$\pm$5.89 & 79.73$\pm$6.87 \\
 \midrule

        DHYPR$_{\text{F}}$ & 10.18$\pm$1.21 & 13.66$\pm$1.47 & 20.93$\pm$2.41 & 3.15$\pm$0.57 & 87.35$\pm$1.54 & 88.83$\pm$0.95 & 76.94$\pm$0.63 \\
        
        DHYPR$_{\text{D}}$ & 0.16$\pm$0.14 & 0.52$\pm$0.83 & 1.63$\pm$1.23 & 0.28$\pm$0.06 & 58.85$\pm$1.39 & 56.65$\pm$0.62 & 53.91$\pm$0.66 \\  \midrule
        
        DiGAE$_{\text{F}}$ & 27.79$\pm$3.85 & 43.32$\pm$3.36 & 55.05$\pm$2.36 & 9.38$\pm$2.47 & 97.98$\pm$0.08 & 97.99$\pm$0.10 & 91.77$\pm$0.18 \\
        DiGAE$_{\text{D}}$ & 16.55$\pm$1.20 & 26.17$\pm$2.03 & 34.60$\pm$2.09 & 5.36$\pm$1.66 & 93.14$\pm$0.14 & 93.76$\pm$0.11 & 83.23$\pm$0.34 \\ \midrule

        SDGAE$_{\text{F}}$ &\hig{1}{40.89$\pm$3.86} & \hig{1}{55.76$\pm$4.08} & \hig{2}{68.84$\pm$2.35} & \hig{1}{14.82$\pm$4.22} &\hig{1}{99.25$\pm$0.05} & \hig{1}{99.16$\pm$0.06} & \hig{2}{96.16$\pm$0.14} \\
        SDGAE$_{\text{D}}$ & 24.76$\pm$3.46 & 38.5$\pm$1.66 & 50.96$\pm$2.32 & 9.16$\pm$1.99 & 98.07$\pm$0.15 & 97.98$\pm$0.12 & 93.57$\pm$0.35 \\

        \bottomrule
    \end{tabular}}
\end{table}

\clearpage
\hypertarget{app_complete_res_computers}{}
\subsection{Results on Computers}\label{app_complete_res_computers}
%Table~\ref{app_tb_computers} shows the results of DirLinkBench on Computers.
\begin{table}[ht]
    \centering
    \caption{Benchmark Results on Computers. For all methods, $_{\text{F}}$ indicates the use of original node features as input, while $_{\text{D}}$ indicates the use of in/out degrees as input. Results ranked \hig{1}{first} and \hig{2}{second} are highlighted.}
    \label{app_tb_computers}
    \resizebox{\textwidth}{!}{
    \begin{tabular}{lccccccc}
        \toprule
        Model & Hits@20 & Hits@50 & Hits@100 & MRR & AUC & AP & ACC \\
        \midrule
        STRAP & \hig{2}{24.35$\pm$3.75} &\hig{2}{38.14$\pm$3.77} & \hig{2}{51.87$\pm$2.07} & \hig{2}{7.44$\pm$1.98} & 98.19$\pm$0.03 & 98.32$\pm$0.03 & 93.43$\pm$0.07 \\
        
        ODIN & 4.42$\pm$1.18 & 8.41$\pm$1.27 & 12.98$\pm$1.47 & 1.46$\pm$0.63 & 89.35$\pm$0.09 & 89.15$\pm$0.35 & 81.73$\pm$0.10  \\
        
        ELTRA & 4.82$\pm$0.75 & 8.66$\pm$1.38 & 14.74$\pm$1.55 & 1.61$\pm$0.52 & 95.63$\pm$0.10 & 95.11$\pm$0.14 & 89.30$\pm$0.15  \\ \midrule
        
        MLP$_{\text{F}}$ & 5.51$\pm$0.72 & 9.31$\pm$0.90 & 14.26$\pm$0.88 & 1.63$\pm$0.42 & 92.83$\pm$0.36 & 91.86$\pm$0.39 & 85.33$\pm$0.57 \\ 
        MLP$_{\text{D}}$ & 6.97$\pm$1.22 & 12.2$\pm$0.88 & 17.57$\pm$0.85 & 2.76$\pm$0.75 & 87.48$\pm$0.16 & 88.69$\pm$0.15 & 78.75$\pm$0.36  \\ \midrule
        
        GCN$_{\text{F}}$ & 19.32$\pm$2.69 & 31.47$\pm$1.81 & 43.77$\pm$1.75 & 7.26$\pm$1.64 & 98.97$\pm$0.06 & \hig{2}{98.80$\pm$0.06} & \hig{2}{95.69$\pm$0.13} \\
        GCN$_{\text{D}}$ & 10.59$\pm$1.40 & 17.48$\pm$1.07 & 24.59$\pm$1.01 & 4.33$\pm$1.26 & 94.41$\pm$0.10 & 94.25$\pm$0.12 & 87.00$\pm$0.13 \\ \midrule

        GAT$_{\text{F}}$ & 14.89$\pm$3.24 & 27.53$\pm$2.48 & 40.74$\pm$3.22 & 3.37$\pm$0.92 &\hig{2}{98.99$\pm$0.11} & 98.76$\pm$0.15 & \hig{1}{95.78$\pm$0.26} \\
        GAT$_{\text{D}}$ & 7.16$\pm$1.53 & 14.49$\pm$1.54 & 21.98$\pm$1.04 & 2.36$\pm$0.69 & 95.20$\pm$0.44 & 94.81$\pm$0.47 & 88.14$\pm$0.67 \\ \midrule

        APPNP$_{\text{F}}$ & 12.40$\pm$1.24 & 21.71$\pm$1.13 & 32.24$\pm$1.40 & 4.86$\pm$1.06 & 98.21$\pm$0.08 & 97.90$\pm$0.11 & 94.01$\pm$0.16 \\ 
        APPNP$_{\text{D}}$ & 9.54$\pm$1.53 & 15.36$\pm$1.20 & 21.92$\pm$1.32 & 3.99$\pm$0.83 & 93.84$\pm$0.35 & 93.49$\pm$0.38 & 85.76$\pm$0.52 \\\midrule

        DGCN$_{\text{F}}$ & 17.74$\pm$2.16 & 27.81$\pm$1.84 & 39.92$\pm$1.94 & 6.51$\pm$1.53 & 98.78$\pm$0.10 & 98.59$\pm$0.11 & 95.22$\pm$0.20 \\
        DGCN$_{\text{D}}$ & 11.12$\pm$1.50 & 17.79$\pm$1.66 & 25.20$\pm$1.87 & 4.06$\pm$0.70 & 95.54$\pm$0.50 & 95.30$\pm$0.53 & 88.72$\pm$0.74 \\ \midrule

        DiGCN$_{\text{F}}$ & 11.68$\pm$1.84 & 19.02$\pm$2.06 & 27.51$\pm$1.67 & 4.61$\pm$0.71 & 97.87$\pm$0.24 & 97.47$\pm$0.27 & 93.44$\pm$0.54 \\
        DiGCN$_{\text{D}}$ & 10.98$\pm$1.53 & 17.76$\pm$1.37 & 24.46$\pm$1.51 & 4.69$\pm$1.09 & 94.86$\pm$0.11 & 94.75$\pm$0.12 & 87.59$\pm$0.17 \\ \midrule
        
        DiGCNIB$_{\text{F}}$ & 13.41$\pm$2.95 & 22.54$\pm$1.79 & 32.44$\pm$1.85 & 4.86$\pm$0.80 & 98.46$\pm$0.14 & 98.15$\pm$0.17 & 94.61$\pm$0.31 \\
        DiGCNIB$_{\text{D}}$ & 10.70$\pm$0.84 & 16.69$\pm$1.41 & 24.74$\pm$1.41 & 5.10$\pm$1.08 & 96.50$\pm$0.09 & 96.19$\pm$0.11 & 90.77$\pm$0.15  \\ \midrule
        
        DirGNN$_{\text{F}}$ & 13.95$\pm$1.66 & 23.94$\pm$1.26 & 35.65$\pm$1.30 & 5.02$\pm$0.60 & 98.56$\pm$0.05 & 98.28$\pm$0.07 & 94.68$\pm$0.14 \\
        DirGNN$_{\text{D}}$ & 13.09$\pm$0.90 & 21.84$\pm$1.54 & 30.70$\pm$0.98 & 6.14$\pm$1.58 & 96.70$\pm$0.08 & 96.64$\pm$0.07 & 91.08$\pm$0.13  \\
        \midrule
        
        MagNet$_{\text{F}}$ & 5.02$\pm$0.60 & 8.49$\pm$0.48 & 12.66$\pm$0.62 & 1.74$\pm$0.66 & 89.18$\pm$0.08 & 88.99$\pm$0.10 & 81.43$\pm$0.08 \\
        MagNet$_{\text{D}}$ & 4.50$\pm$0.76 & 8.15$\pm$0.89 & 12.85$\pm$0.59 & 0.97$\pm$0.22 & 89.37$\pm$0.03 & 89.25$\pm$0.05 & 81.61$\pm$0.11 \\ \midrule

        DUPLEX$_{\text{F}}$ & 7.36$\pm$0.85 & 13.19$\pm$0.97 & 17.90$\pm$0.71 & 2.27$\pm$0.63 & 92.05$\pm$0.22 & 91.45$\pm$0.29 & 85.65$\pm$0.27 \\
        DUPLEX$_{\text{D}}$ & 5.92$\pm$1.83 & 9.04$\pm$4.80 & 14.56$\pm$5.51 & 1.48$\pm$0.55 & 87.00$\pm$4.97 & 86.79$\pm$4.33 & 78.90$\pm$5.65 \\ \midrule

        DiGAE$_{\text{F}}$ & 19.65$\pm$1.33 & 31.16$\pm$1.62 & 41.55$\pm$1.62 & 5.34$\pm$1.18 & 97.29$\pm$0.13 & 97.12$\pm$0.44 & 89.52$\pm$0.15 \\
        DiGAE$_{\text{D}}$ & 11.94$\pm$0.96 & 19.38$\pm$1.60 & 26.53$\pm$1.20 & 3.58$\pm$1.20 & 92.86$\pm$0.28 & 93.51$\pm$0.20 & 82.11$\pm$0.32 \\ \midrule

        SDGAE$_{\text{F}}$ &\hig{1}{27.07$\pm$2.34} &\hig{1}{41.37$\pm$1.61} & \hig{1}{53.79$\pm$1.56} &\hig{1}{ 8.41$\pm$1.89} & \hig{1}{99.07$\pm$0.04} & \hig{1}{99.00$\pm$0.03} &95.66$\pm$0.12 \\
        
        SDGAE$_{\text{D}}$& 15.18$\pm$2.22 & 24.02$\pm$1.53 & 33.51$\pm$1.16 & 5.73$\pm$1.33 & 97.44$\pm$0.12 & 97.32$\pm$0.11 & 92.26$\pm$0.24 \\

        \bottomrule
    \end{tabular}}
\end{table}

\clearpage
\hypertarget{app_complete_res_wiki}{}
\subsection{Results on WikiCS}\label{app_complete_res_wiki}
%Table~\ref{app_tb_wikics} shows the results of DirLinkBench on Wikics.
\begin{table}[ht]
    \centering
    \caption{Benchmark Results on WikiCS. For all methods, $_{\text{F}}$ indicates the use of original node features as input, while $_{\text{D}}$ indicates the use of in/out degrees as input. Results ranked \hig{1}{first} and \hig{2}{second} are highlighted.}
    \label{app_tb_wikics}
    \resizebox{\textwidth}{!}{
    \begin{tabular}{lccccccc}
        \toprule
        Model & Hits@20 & Hits@50 & Hits@100 & MRR & AUC & AP & ACC \\
        \midrule
        STRAP &\hig{1}{64.97$\pm$1.52} &\hig{1}{71.10$\pm$1.13} & \hig{1}{76.27$\pm$0.92} & \hig{1}{37.29$\pm$9.42} &\hig{1}{98.66$\pm$0.03} &\hig{1}{98.91$\pm$0.02} &\hig{1}{94.57$\pm$0.06} \\
        
        ODIN & 3.41$\pm$0.60 & 6.24$\pm$0.63 & 9.83$\pm$0.47 & 1.17$\pm$0.35 & 92.86$\pm$0.04 & 91.90$\pm$0.10 & 86.39$\pm$0.08  \\
        
        ELTRA & 3.84$\pm$0.49 & 6.62$\pm$0.55 & 9.88$\pm$0.70 & 1.42$\pm$0.33 & 92.66$\pm$0.19 & 92.19$\pm$0.23 & 85.73$\pm$0.28  \\ \midrule
        
        MLP$_\text{F}$ & 0.24$\pm$0.09 & 0.71$\pm$0.40 & 1.21$\pm$0.25 & 0.15$\pm$0.07 & 71.90$\pm$0.54 & 70.86$\pm$0.68 & 66.26$\pm$0.67 \\ 
        MLP$_\text{D}$ & 4.04$\pm$0.72 & 7.92$\pm$0.61 & 12.99$\pm$0.68 & 1.63$\pm$0.20 & 92.12$\pm$0.10 & 91.90$\pm$0.19 & 84.65$\pm$0.22 \\ \midrule
        
        GCN$_\text{F}$ & 6.10$\pm$1.85 & 11.25$\pm$1.86 & 18.05$\pm$1.43 & 2.07$\pm$0.49 & 95.86$\pm$0.27 & 95.41$\pm$0.45 & 89.85$\pm$0.35  \\
        GCN$_\text{D}$ & 18.15$\pm$2.49 & 30.21$\pm$2.51 & 38.37$\pm$1.51 & 6.09$\pm$2.16 & 95.97$\pm$0.08 & 96.23$\pm$0.08 & 89.58$\pm$0.09 \\ \midrule
        
        GAT$_\text{F}$ & 1.83$\pm$0.54 & 3.52$\pm$2.21 & 5.60$\pm$1.17 & 0.83$\pm$0.31 & 73.18$\pm$3.59 & 74.81$\pm$4.19 & 54.16$\pm$6.34 \\
        GAT$_\text{D}$ & 24.13$\pm$4.10 & 34.32$\pm$4.41 & 40.47$\pm$4.10 & 7.67$\pm$2.07 & 95.72$\pm$0.27 & 96.06$\pm$0.33 & 88.90$\pm$0.36  \\ \midrule

        APPNP$_\text{F}$ & 3.71$\pm$0.46 & 6.66$\pm$0.76 & 11.11$\pm$1.09 & 1.64$\pm$0.33 & 92.76$\pm$0.63 & 92.11$\pm$0.63 & 85.56$\pm$0.08 \\ 
        APPNP$_\text{D}$ & 7.60$\pm$1.75 & 12.76$\pm$3.01 & 20.23$\pm$1.72 & 2.75$\pm$0.70 & 94.12$\pm$0.09 & 93.89$\pm$0.12 & 87.51$\pm$0.14 \\ \midrule
        
        DGCN$_\text{F}$ & 5.84$\pm$1.79 & 10.12$\pm$3.32 & 15.88$\pm$5.12 & 2.04$\pm$0.50 & 95.98$\pm$0.65 & 95.45$\pm$0.80 & 89.95$\pm$0.96 \\
        DGCN$_\text{D}$ & 8.35$\pm$3.46 & 16.51$\pm$2.99 & 25.91$\pm$4.10 & 2.88$\pm$1.11 & 96.22$\pm$0.32 & 96.04$\pm$0.43 & 90.13$\pm$0.37 \\ \midrule

        DiGCN$_\text{F}$ & 3.63$\pm$0.69 & 6.77$\pm$0.98 & 10.24$\pm$0.88 & 1.58$\pm$0.46 & 92.55$\pm$1.53 & 91.63$\pm$1.62 & 82.60$\pm$2.14 \\
        DiGCN$_\text{D}$ & 10.08$\pm$1.33 & 16.32$\pm$2.16 & 25.31$\pm$1.84 & 3.85$\pm$0.98 & 95.59$\pm$0.12 & 95.57$\pm$0.12 & 88.89$\pm$0.14 \\ \midrule
        
        DiGCNIB$_\text{F}$ & 5.36$\pm$0.58 & 8.28$\pm$1.20 & 13.61$\pm$1.18 & 1.81$\pm$0.48 & 94.00$\pm$0.33 & 93.31$\pm$0.39 & 84.49$\pm$1.62 \\
        DiGCNIB$_\text{D}$& 12.01$\pm$2.95 & 20.99$\pm$1.75 & 28.28$\pm$2.44 & 3.96$\pm$1.16 & 96.36$\pm$0.07 & 96.30$\pm$0.08 & 90.72$\pm$0.10 \\ \midrule
        
        DirGNN$_\text{F}$ & 11.76$\pm$3.31 & 23.90$\pm$3.31 & 33.28$\pm$2.84 & 4.82$\pm$1.77 & 97.09$\pm$0.13 & 97.04$\pm$0.16 & 91.55$\pm$0.25 \\ 
        DirGNN$_\text{D}$ & 28.16$\pm$2.09 & 40.94$\pm$1.19 & 50.48$\pm$0.85 & \hig{2}{12.08$\pm$2.05} & 97.13$\pm$0.09 & 97.33$\pm$0.09 & 91.28$\pm$0.14 \\\midrule
        
        MagNet$_\text{F}$ & 3.41$\pm$0.35 & 6.10$\pm$0.45 & 9.25$\pm$0.57 & 1.42$\pm$0.22 & 92.57$\pm$0.08 & 91.54$\pm$0.10 & 86.06$\pm$0.11 \\
        MagNet$_\text{D}$ & 4.13$\pm$0.46 & 6.57$\pm$0.34 & 10.81$\pm$0.46 & 1.26$\pm$0.37 & 93.06$\pm$0.06 & 92.18$\pm$0.07 & 86.59$\pm$0.06 \\ \midrule
        
        DUPLEX$_{\text{F}}$ & 2.97$\pm$0.52 & 5.54$\pm$0.63 & 8.52$\pm$0.60 & 0.89$\pm$0.22 & 90.92$\pm$0.12 & 90.06$\pm$0.45 & 83.82$\pm$0.23 \\
        DUPLEX$_{\text{D}}$ & 1.09$\pm$0.92 & 1.53$\pm$3.12 & 5.45$\pm$0.19 & 1.03$\pm$0.08 & 90.93$\pm$0.04 & 90.37$\pm$0.23 & 83.81$\pm$0.11 \\ \midrule
        
        DiGAE$_{\text{F}}$ & 7.01$\pm$1.78 & 11.54$\pm$1.11 & 18.17$\pm$1.27 & 2.18$\pm$0.78 & 93.47$\pm$1.04 & 93.20$\pm$1.16 & 76.38$\pm$0.21  \\
        DiGAE$_{\text{D}}$ & 10.6$\pm$1.89 & 19.69$\pm$1.98 & 29.21$\pm$1.36 & 4.59$\pm$0.88 & 93.46$\pm$0.22 & 94.47$\pm$0.15 & 82.53$\pm$0.48 \\ \midrule

        SDGAE$_{\text{F}}$& 8.54$\pm$3.42 & 19.60$\pm$5.04 & 29.95$\pm$5.80 & 2.35$\pm$0.91 & 96.64$\pm$1.23 & 96.58$\pm$1.20 & 90.98$\pm$1.52  \\
        SDGAE$_{\text{D}}$&\hig{2}{33.04$\pm$3.27} & \hig{2}{47.62$\pm$1.74} &\hig{2}{54.67$\pm$2.50} &11.78$\pm$4.11 &\hig{2}{97.23$\pm$0.07} & \hig{2}{97.58$\pm$0.06} &\hig{2}{92.24$\pm$0.12}  \\
        \bottomrule
    \end{tabular}}
\end{table}

\clearpage
\hypertarget{app_complete_res_slash}{}
\subsection{Results on Slashdot}\label{app_complete_res_slash}
%Table~\ref{app_tb_slash} shows the results of DirLinkBench on Slashdot.
\begin{table}[h]
    \centering
    \caption{Benchmark Results on Slashdot. For all methods, $_{\text{R}}$ indicates the use of random node features as input, while $_{\text{D}}$ indicates the use of in/out degrees as input. Results ranked \hig{1}{first} and \hig{2}{second} are highlighted.}
    \label{app_tb_slash}
    \resizebox{\textwidth}{!}{
    \begin{tabular}{lccccccc}
        \toprule
        Model & Hits@20 & Hits@50 & Hits@100 & MRR & AUC & AP & ACC \\
        \midrule
        STRAP & 19.10$\pm$1.06 & 25.39$\pm$1.43 & 31.43$\pm$1.21 & \hig{1}{9.82$\pm$1.82} & 94.74$\pm$0.05 & 95.13$\pm$0.05 & 88.19$\pm$0.08  \\
        
        ODIN & 14.97$\pm$1.40 & 24.91$\pm$1.19 & 34.17$\pm$1.19 & 4.44$\pm$1.59 & 96.58$\pm$0.07 & 96.75$\pm$0.06 & 90.39$\pm$0.10  \\
        
        ELTRA & 18.02$\pm$2.11 & 26.31$\pm$0.95 & 33.44$\pm$1.00 & 5.53$\pm$1.77 & 94.65$\pm$0.03 & 95.23$\pm$0.04 & 88.11$\pm$0.11 \\ \midrule
        
        MLP$_{\text{R}}$ & 4.25$\pm$0.71 & 7.26$\pm$0.74 & 11.31$\pm$0.70 & 1.28$\pm$0.33 & 72.86$\pm$0.37 & 76.72$\pm$0.21 & 66.16$\pm$0.26   \\ 
        MLP$_{\text{D}}$ & 14.16$\pm$5.22 & 24.01$\pm$0.79 & 32.97$\pm$0.51 & 4.14$\pm$1.71 & 95.84$\pm$0.07 & 96.21$\pm$0.05 & 89.62$\pm$0.11 \\ \midrule
        
        GCN$_{\text{R}}$ & 12.52$\pm$1.30 & 21.03$\pm$1.62 & 29.04$\pm$0.95 & 3.03$\pm$0.73 & 95.58$\pm$0.13 & 95.69$\pm$0.13 & 89.46$\pm$0.12   \\
        GCN$_{\text{D}}$ & 16.28$\pm$1.59 & 24.51$\pm$1.63 & 33.16$\pm$1.22 & 5.54$\pm$2.04 & 95.90$\pm$0.07 & 96.17$\pm$0.06 & 89.75$\pm$0.17  \\ \midrule
        
        GAT$_{\text{R}}$ & 14.82$\pm$2.70 & 22.19$\pm$2.78 & 30.16$\pm$3.11 & 5.11$\pm$1.53 & 96.26$\pm$0.18 & 96.45$\pm$0.20 & 87.14$\pm$1.03  \\
        GAT$_{\text{D}}$ & 12.39$\pm$1.47 & 19.54$\pm$1.89 & 26.65$\pm$1.98 & 4.53$\pm$0.78 & 95.01$\pm$0.34 & 95.25$\pm$0.45 & 88.01$\pm$0.49 \\ \midrule

        APPNP$_{\text{R}}$ & 14.83$\pm$1.18 & 22.75$\pm$1.45 & 31.25$\pm$1.14 & 4.56$\pm$1.37 & 95.36$\pm$0.07 & 95.72$\pm$0.06 & 88.76$\pm$0.09  \\ 
        APPNP$_{\text{D}}$ & 15.00$\pm$5.47 & 24.34$\pm$1.47 & 33.76$\pm$1.05 & 5.86$\pm$2.78 & 96.21$\pm$0.06 & 96.43$\pm$0.05 & 90.07$\pm$0.10  \\ \midrule

        %DGCN & TO & TO & TO & TO & TO & TO & TO \\
        %DiGCN & TO & TO & TO & TO & TO & TO & TO \\
        %DiGCNIB & TO & TO & TO & TO & TO & TO & TO \\
        DirGNN$_{\text{R}}$ & 18.72$\pm$1.93 & 28.52$\pm$1.09 & 37.41$\pm$1.37 & 6.19$\pm$2.04 & 96.67$\pm$0.05 & 96.89$\pm$0.04 & 90.24$\pm$0.12  \\
        DirGNN$_{\text{D}}$ & 20.55$\pm$2.85 & 31.20$\pm$1.18 & 41.74$\pm$1.15 & 7.52$\pm$3.24 &\hig{1}{96.95$\pm$0.05} & \hig{1}{97.14$\pm$0.06} &\hig{1}{ 90.65$\pm$0.13}  \\ \midrule
        
        MagNet$_{\text{R}}$ & 9.16$\pm$1.26 & 19.58$\pm$1.37 & 28.50$\pm$1.78 & 1.98$\pm$0.25 & 96.31$\pm$0.06 & 96.38$\pm$0.06 & 90.04$\pm$0.13 \\
        MagNet$_{\text{D}}$ & 12.55$\pm$0.75 & 22.34$\pm$0.42 & 31.98$\pm$1.06 & 2.83$\pm$0.51 & 96.57$\pm$0.09 & 96.69$\pm$0.10 & 90.45$\pm$0.09 \\ \midrule
        
        DUPLEX$_{\text{R}}$ &5.67$\pm$1.85	&11.49$\pm$3.36	&18.42$\pm$2.59	&1.81$\pm$0.83	&94.36$\pm$3.25	&94.48$\pm$2.76	&85.42$\pm$3.42\\
        DUPLEX$_{\text{D}}$ & 2.51$\pm$0.64 & 5.95$\pm$1.11 & 9.39$\pm$2.71 & 0.51$\pm$0.01 & 80.57$\pm$3.85 & 86.52$\pm$1.50 & 77.67$\pm$2.24 \\ \midrule
        
        DiGAE$_{\text{R}}$ & 18.89$\pm$1.71 & 27.69$\pm$1.41 & 36.57$\pm$1.32 & 5.49$\pm$2.96 & 95.26$\pm$0.29 & 96.13$\pm$0.19 & 84.27$\pm$0.26  \\
        DiGAE$_{\text{D}}$ &\hig{1}{23.68$\pm$0.94} &\hig{1}{33.97$\pm$1.06} &\hig{2}{41.95$\pm$0.93} & 5.54$\pm$1.51 & 94.30$\pm$0.29 & 95.80$\pm$0.12 & 85.67$\pm$0.28 \\ \midrule

        SDGAE$_{\text{R}}$ &18.24$\pm$2.05 & 28.47$\pm$1.97 & 37.34$\pm$0.68 & 5.51$\pm$1.65 & 95.96$\pm$0.07 & 96.31$\pm$0.03 & 90.11$\pm$0.11  \\
        SDGAE$_{\text{D}}$ &\hig{2}{23.57$\pm$2.11} &\hig{2}{33.75$\pm$1.48} & \hig{1}{42.42$\pm$1.15} &\hig{2}{8.41$\pm$3.80} & \hig{2}{96.70$\pm$0.10} & \hig{2}{97.06$\pm$0.08} & \hig{1}{91.05$\pm$0.20} \\
        
        \bottomrule
    \end{tabular}}
\end{table}

\clearpage
\hypertarget{app_complete_res_epinion}{}
\subsection{Results on Epinions}\label{app_complete_res_epinion}
%Table~\ref{app_tb_epinion} shows the results of DirLinkBench on Epinions.
\begin{table}[ht]
    \centering
    \caption{Benchmark Results on Epinions. For all methods, $_{\text{R}}$ indicates the use of random node features as input, while $_{\text{D}}$ indicates the use of in/out degrees as input. Results ranked \hig{1}{first} and \hig{2}{second} are highlighted.}
    \label{app_tb_epinion}
    \resizebox{\textwidth}{!}{
    \begin{tabular}{lccccccc}
        \toprule
        Model & Hits@20 & Hits@50 & Hits@100 & MRR & AUC & AP & ACC \\
        \midrule
        STRAP & \hig{1}{44.66$\pm$1.68} &  \hig{1}{53.48$\pm$0.86} &  \hig{1}{58.99$\pm$0.82} &  \hig{1}{21.18$\pm$6.31} & 96.62$\pm$0.06 & 97.60$\pm$0.04 & 91.89$\pm$0.06 \\
        
        ODIN & 11.85$\pm$3.33 & 25.99$\pm$1.79 & 36.91$\pm$0.47 & 3.22$\pm$0.80 & 97.72$\pm$0.03 & 97.91$\pm$0.03 & 92.42$\pm$0.07  \\
        
        ELTRA & 16.89$\pm$1.27 & 28.37$\pm$1.53 & 41.63$\pm$2.53 & 5.81$\pm$1.10 & 96.19$\pm$0.04 & 97.47$\pm$0.03 & 90.40$\pm$0.13 \\ \midrule
        
        MLP$_\text{R}$ & 3.84$\pm$0.65 & 7.02$\pm$0.40 & 10.18$\pm$0.67 & 1.18$\pm$0.36 & 78.44$\pm$0.25 & 80.67$\pm$0.14 & 67.83$\pm$1.93  \\ 
        MLP$_\text{D}$ & 15.84$\pm$3.61 & 34.11$\pm$2.04 & 44.59$\pm$1.62 & 4.35$\pm$1.64 & 97.85$\pm$0.08 & 98.02$\pm$0.07 & 92.56$\pm$0.45  \\ \midrule
        
        GCN$_\text{R}$ & 18.26$\pm$2.56 & 30.18$\pm$1.71 & 40.64$\pm$1.53 & 4.04$\pm$1.10 & 96.90$\pm$0.04 & 97.54$\pm$0.03 & 92.10$\pm$0.24  \\
        GCN$_\text{D}$& 12.40$\pm$7.59 & 30.79$\pm$9.24 & 46.10$\pm$1.37 & 3.12$\pm$0.71 & 97.83$\pm$0.09 & 98.15$\pm$0.05 &\hig{2}{94.17$\pm$0.08} \\ \midrule

        GAT$_\text{R}$ & 19.65$\pm$3.52 & 31.90$\pm$3.56 & 43.65$\pm$4.88 & 6.04$\pm$2.16 & 98.35$\pm$0.11 & \hig{2}{ 98.50$\pm$0.11} & 92.05$\pm$1.30  \\
        GAT$_\text{D}$ & 18.18$\pm$4.11 & 27.18$\pm$3.95 & 36.76$\pm$5.74 & 7.98$\pm$1.92 & 97.61$\pm$0.29 & 97.81$\pm$0.22 & 92.92$\pm$0.37 \\ \midrule
        
        APPNP$_\text{R}$  & 17.86$\pm$2.53 & 27.89$\pm$1.24 & 39.06$\pm$1.26 & 4.88$\pm$4.14 & 97.70$\pm$0.04 & 97.92$\pm$0.02 & 92.84$\pm$0.06  \\ 
        APPNP$_\text{D}$& 18.46$\pm$3.51 & 30.84$\pm$1.84 & 41.99$\pm$1.23 & 6.41$\pm$3.73 &\hig{2}{98.36$\pm$0.06} & 98.48$\pm$0.06 & 94.17$\pm$0.16  \\ \midrule
        %DGCN & TO & TO & TO & TO & TO & TO & TO \\
        %DiGCN & TO & TO & TO & TO & TO & TO & TO \\
        %DiGCNIB & TO & TO & TO & TO & TO & TO & TO \\
      
        DirGNN$_{\text{R}}$ & 25.66$\pm$3.33 & 39.28$\pm$1.96 & 50.10$\pm$2.06 & 7.03$\pm$2.70 & 98.25$\pm$0.03 & 98.46$\pm$0.03 & 93.99$\pm$0.05 \\
        DirGNN$_{\text{D}}$ & 21.35$\pm$2.89 & 34.06$\pm$2.53 & 46.01$\pm$2.07 & 6.12$\pm$2.54 & 98.03$\pm$0.03 & 98.26$\pm$0.02 & 93.48$\pm$0.06 \\ \midrule

        MagNet$_{\text{R}}$ & 6.41$\pm$1.57 & 12.95$\pm$1.51 & 22.12$\pm$1.27 & 1.62$\pm$0.35 & 97.60$\pm$0.03 & 97.69$\pm$0.03 & 92.79$\pm$0.05  \\
        MagNet$_{\text{D}}$ & 7.68$\pm$1.00 & 16.30$\pm$2.36 & 28.01$\pm$1.72 & 2.53$\pm$0.57 & 97.71$\pm$0.03 & 97.86$\pm$0.04 & 92.92$\pm$0.05  \\ \midrule
        
        DUPLEX$_{\text{R}}$ & 3.76$\pm$1.94 & 8.38$\pm$4.39 & 16.50$\pm$4.34 & 1.85$\pm$0.39 & 92.11$\pm$2.25 & 93.78$\pm$3.69 & 88.20$\pm$3.86  \\
        DUPLEX$_{\text{D}}$ & 2.43$\pm$0.86 & 6.74$\pm$0.45 & 12.35$\pm$2.64 & 0.46$\pm$0.08 & 90.61$\pm$1.76 & 88.72$\pm$3.26 & 81.82$\pm$3.74  \\ \midrule
        
        DiGAE$_{\text{R}}$ & 29.11$\pm$3.51 & 43.25$\pm$1.68 & 53.27$\pm$1.17 & 8.85$\pm$2.81 & 97.11$\pm$0.19 & 97.78$\pm$0.11 & 89.16$\pm$0.24   \\
        DiGAE$_{\text{D}}$ & 22.56$\pm$9.23 & 43.19$\pm$2.97 & 55.14$\pm$1.96 & 5.33$\pm$1.78 & 96.47$\pm$0.18 & 97.37$\pm$0.10 & 90.17$\pm$0.14  \\ \midrule

        SDGAE$_{\text{R}}$ & 21.88$\pm$2.17 & 35.28$\pm$2.35 & 45.04$\pm$2.18 & 6.54$\pm$1.94 & 98.11$\pm$0.03 & 98.35$\pm$0.03 & 93.83$\pm$0.07 \\
        SDGAE$_{\text{D}}$ &\hig{2}{32.81$\pm$2.67} &\hig{2}{45.61$\pm$1.92} &\hig{2}{55.91$\pm$1.77} &\hig{2}{11.62$\pm$2.86} &  \hig{1}{98.43$\pm$0.07} &\hig{1}{98.64$\pm$0.04} &\hig{1}{94.33$\pm$0.11}  \\
        
        \bottomrule
    \end{tabular}}
\end{table}
