# Supplementary material for: Rethinking Link Prediction for Directed Graphs
Source: arXiv:2502.05724 source file (2025-05-21)
Supplement: Supplementary file 2 [file appendix_benchmark.tex]

\hypertarget{app:experiments}{} 
\section{More Details of DirLinkBench} \label{app:experiments}

\hypertarget{app_dataset_baseline}{} 
\subsection{Datasets and baselines}\label{app_dataset_baseline}
\textbf{Datasets Details.}
Table~\ref{dataset_info} summarizes the statistical characteristics of seven directed graphs. Avg. Degree indicates average node connectivity and \%Directed Edges reflects inherent directionality. Detailed descriptions:
\begin{itemize}
    \item Cora-ML~\cite{mccallum2000cora_ml,bojchevski2018cora_ml} and CiteSeer~\cite{sen2008citeseer} are two citation networks. 
    Nodes represent academic papers, and edges represent directed citation relationships.
    \item Photo and Computers~\cite{shchur2018computerandphoto} are two Amazon co-purchasing networks. Nodes denote products, and directed edges denote the sequential purchase relationships.
    \item WikiCS~\cite{mernyei2020wiki} is a weblink network where nodes represent computer science articles from Wikipedia and directed edges correspond to hyperlinks between articles.
    \item Slashdot~\cite{ordozgoiti2020slash} and Epinions~\cite{massa2005epinion} are two social networks, where nodes represent users. Edges in Slashdot indicate directed social interactions between users, and edges in Epinions represent unidirectional trust relationships between users.
\end{itemize}

\begin{table*}[h]
\centering
\caption{Statistics of DirLinkBench datasets.}
\resizebox{\textwidth}{!}{
\begin{tabular}{lrrrrcr}
\toprule
Datasets & \#Nodes & \#Edges &Avg. Degree & \#Features & \%Directed Edges &Description \\ \midrule
Cora-ML & 2,810 & 8,229 & 5.9 &2,879 & 93.97 & citation network \\

CiteSeer & 2,110 & 3,705 & 3.5 & 3,703 & 98.00 & citation network \\
Photo & 7,487 & 143,590 & 38.4 & 745 & 65.81 & co-purchasing network \\
Computers & 13,381 & 287,076 & 42.9 & 767 & 71.23 & co-purchasing network \\
WikiCS & 11,311 & 290,447 & 51.3 & 300 & 48.43 & weblink network \\
Slashdot & 74,444 & 424,557 & 11.4 &- & 80.17 & social network \\
Epinions & 100,751 & 708,715 & 14.1 &- & 65.04 & social network \\
\bottomrule
\end{tabular}}
\label{dataset_info}
\end{table*}

\textbf{Baseline Implementations}. For MLP, GCN, GAT, and APPNP, we use the PyTorch Geometric (PyG) library~\cite{pyg} implementations. For DCN, DiGCN, and DiGCNIB, we rely on the PyTorch Geometric Signed Directed (PyGSD) library~\cite{dpyg} implementations. For other baselines, we use the original code released by the authors. Here are the links to each repository.
\begin{itemize}[topsep=0pt, partopsep=0pt]
    \item Pytorch Geometric library:
    \href{https://github.com/pyg-team/pytorch_geometric/tree/master/benchmark}{https://github.com/pyg-team/pytorch\_geometric/tree/master/benchmark}
    \item PyTorch Geometric Signed Directed library: \href{https://github.com/SherylHYX/pytorch_geometric_signed_directed}{https://github.com/SherylHYX/pytorch\_geometric\_signed\_directed}
    \item STRAP: \href{https://github.com/yinyuan1227/STRAP-git}{https://github.com/yinyuan1227/STRAP-git}
    \item ODIN: \href{https://github.com/hsyoo32/odin}{https://github.com/hsyoo32/odin} 
    \item ELTRA: \href{https://github.com/mrhhyu/ELTRA}{https://github.com/mrhhyu/ELTRA} 
    %\item \textbf{GravityGAE:}  \href{https://github.com/deezer/gravity_graph_autoencoders}{https://github.com/deezer/gravity\_graph\_autoencoders}
    \item DiGAE:
    \href{https://github.com/gidiko/DiGAE}{https://github.com/gidiko/DiGAE}
    \item DHYPR:
    \href{https://github.com/hongluzhou/dhypr}{https://github.com/hongluzhou/dhypr}
    \item DirGNN:
    \href{https://github.com/emalgorithm/directed-graph-neural-network}{https://github.com/emalgorithm/directed-graph-neural-network}
    \item MagNet:
    \href{https://github.com/matthew-hirn/magnet}{https://github.com/matthew-hirn/magnet}
    %\item \textbf{LightDiC:}
    %\href{https://github.com/xkLi-Allen/LightDiC}{https://github.com/xkLi-Allen/LightDiC}
    \item DUPLEX:
    \href{https://github.com/alipay/DUPLEX}{https://github.com/alipay/DUPLEX}
\end{itemize}
\textbf{Baseline setting}. For STRAP, ODIN, and ELTRA, we use four decoders for selection:  
\(\sigma\bigl(\vs_u^{\top}\vt_v\bigr)\), \(\mathrm{LR}\bigl(\vs_u \odot \vt_v\bigr)\), \(\mathrm{LR}\bigl(\vs_u \|\vt_v\bigr)\), and \(\mathrm{LR}\bigl(\vs_u \| \vs_v \| \vt_u \| \vt_v\bigr)\)~\cite{odin}.  
For embedding generation, we follow the parameter settings specified in their respective papers and refer to the code for further details.
For MLP, GCN, GAT, APPNP, DGCN, DiGCN, DiGCNIB, and DirGNN, we use four combinations of loss functions and decoders for selection: CE loss with \(\mathrm{MLP}\bigl(\vh_u\|\vh_v \bigr)\), BCE loss with \(\mathrm{MLP}\bigl( \vh_u\|\vh_v\bigr)\), BCE loss with \(\mathrm{MLP}\bigl( \vh_u \odot \vh_v\bigr)\), and BCE loss with \(\sigma\bigl( \vh_u^{\top}\vh_v\bigr)\). For MagNet, DUPLEX, DHYPR, and DiGAE, we follow the reported loss function and decoder settings from their respective papers. For all GNNs, we set the number of epochs to 2000 with an early stopping criterion of 200 and run each experiment 10 times to report the mean and standard deviation differences.  
The hyperparameter settings for the baselines are detailed below, where 'hidden' represents the number of hidden units, 'embedding' refers to the embedding dimension, 'undirected' indicates whether an undirected training graph is used, 'lr' stands for the learning rate, and 'wd' denotes weight decay.
\begin{itemize}[topsep=0pt, partopsep=0pt]
    \item MLP: hidden: 64, embedding: 64, layer: 2, lr: \{0.01, 0.005\}, wd:  \{0.0, 5e-4\}.
    \item GCN: hidden: 64, embedding: 64, layer: 2, undirected: \{True, False\}, lr: \{0.01, 0.005\}, wd:  \{0.0, 5e-4\}.
    \item GAT: hidden: 8, heads: 8, embedding: 64, layer: 2,  undirected: \{True, False\}, lr: \{0.01, 0.005\}, wd:  \{0.0, 5e-4\}
    \item APPNP: hidden: 64, embedding: 64, $K$: 10, $\alpha$: \{0.1,0.2\}, undirected: \{True, False\}, lr: \{0.01, 0.005\}, wd:  \{0.0, 5e-4\}.
    \item DGCN: hidden: 64, embedding: 64, lr: \{0.01, 0.005\}, wd:  \{0.0, 5e-4\}.
    \item DiGCN and DiGCNIB: hidden: 64, embedding: 64, $\alpha$: \{0.1,0.2\}, layer: 2, lr: \{0.01, 0.005\}, wd:  \{0.0, 5e-4\}.
    \item DirGNN:  hidden: 64, embedding: 64, layer: 2, $\alpha$: \{0.0, 0.5, 1.0\},  jk: \{'cat','max'\}, normalize: \{True, False\}, lr: \{0.01, 0.005\}, wd:  \{0.0, 5e-4\}.
    \item MagNet: hidden: 64, embedding: 64, layer: 2, $K$: \{1, 2\}, $q$: \{0.05, 0.1, 0.15, 0.2, 0.25\}, lr: \{0.01, 0.005\}, wd:  \{0.0, 5e-4\}.
    \item DUPLEX: hidden: 64, embedding: 64, layer: 3, head: 1, loss weight:\{0.1, 0.3\}, loss decay: \{0.0, 1e-2, 1e-4\}, lr: \{0.01, 0.005\}, wd:  \{0.0, 5e-4\}.
    \item DHYPR: hidden: 64, embedding: 32, proximity: \{1, 2\}, $\lambda$: \{0.01, 0.05, 1, 5\}, lr: \{0.01, 0.001\}, wd:  \{0.0, 0.001\}.
    \item DiGAE: hidden: 64, embedding: 64, single layer: \{True, False\}, $(\alpha,\beta): \{0.0, 0.2, 0.4, 0.6, 0.8\}^2$, lr: \{0.01, 0.005\}, wd:  \{0.0, 5e-4\}.
\end{itemize}

\hypertarget{app_bench_metric}{}
\subsection{Metric description}\label{app_bench_metric}
\textbf{Mean Reciprocal Rank (MRR)} evaluates the capability of models to rank the first correct entity in link prediction tasks. It assigns higher weights to top-ranked predictions by computing the average reciprocal rank of the first correct answer across queries: $\text{MRR} = \frac{1}{|Q|} \sum_{i=1}^{|Q|} \frac{1}{\text{rank}_i}$, where \(|Q|\) is the total number of queries and \(\text{rank}_i\) denotes the position of the first correct answer for the \(i\)-th query. MRR emphasizes early-ranking performance, making it sensitive to improvements in top predictions.

\textbf{Hits@K} measures the proportion of relevant items that appear in the top-$\text{K}$ positions of the ranked list of items. For \(N\) queries, Hits@K$=\frac{1}{N}\sum\nolimits_{i=1}^{N}\mathbf{1}(\text{rank}_i\leq \text{K})$,
where rank$_i$ is the rank of the $i$-th sample and the indicator function $\mathbf{1}$ is 1 if rank$_i \leq \text{K}$, and 0 otherwise. Following the OGB benchmark~\cite{ogb}, link prediction implementations compare each positive sample's score against a set of negative sample scores. A "hit" occurs if the positive sample's score surpasses at least K-1 negative scores, with final results averaged across all queries.

\textbf{Area Under the Curve (AUC)} measures the likelihood that a positive sample is ranked higher than a random negative sample. \(\text{AUC} = \frac{\sum_{i=1}^{M}\sum_{j=1}^{N}\mathbf{1}(s_i^{\text{pos}} > s_j^{\text{neg}})}{M \times N}\), where \(M\) and \(N\) are positive/negative sample counts, \(s_i^{\text{pos}}\) and \(s_j^{\text{neg}}\) their prediction scores. Values approaching 1 indicate perfect separation of positive and negative edges.

\textbf{Average Precision (AP)} is defined as the area under the Precision-Recall (PR) curve. Formally, \(\text{AP} = \sum_{i=1}^{N} (R_i - R_{i-1}) \times P_i,\) where \(P_i\) is the precision at the \(i\)-th threshold, \(R_i\) is the recall at the \(i\)-th threshold, and \(N\) is the number of thresholds considered. 

\textbf{Accuracy (ACC)} measures the proportion of correctly predicted samples among all predictions. Formally, \(\text{ACC} = \frac{TP + TN}{TP + TN + FP + FN},\) where \(TP\), \(TN\), \(FP\), and \(FN\) represent true positives, true negatives, false positives, and false negatives, respectively.

\begin{figure*}[h]
    \centering
   \vspace{-2mm}
   \hspace{-3mm}
   \subfigure[Photo]{
   \label{fig:app_feature_photo}
   \includegraphics[width=57mm]{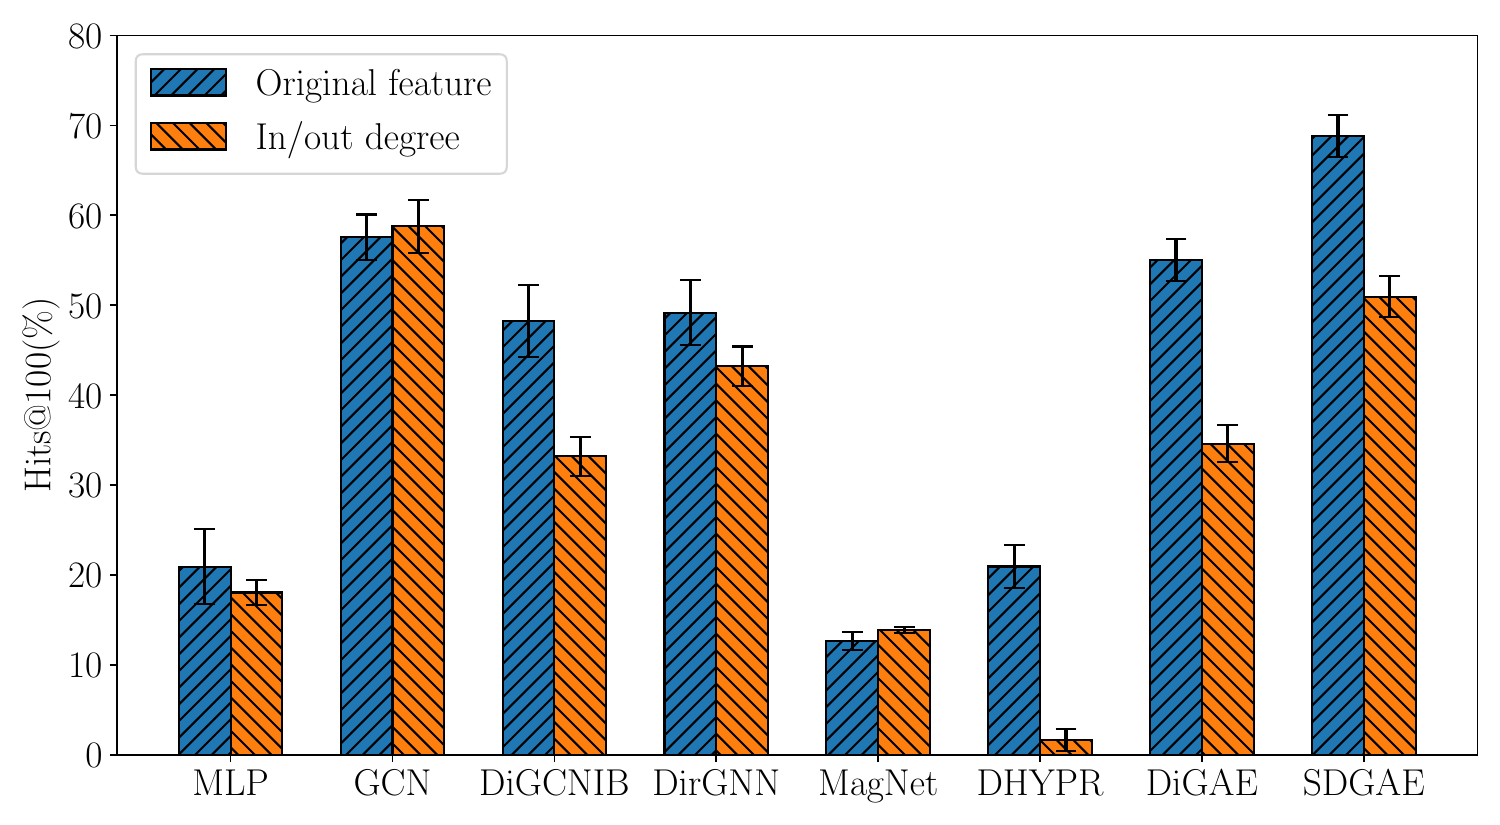}
   }
   \hspace{-5mm}
   \subfigure[WikiCS]{
   \label{fig:app_feature_wiki}
   \includegraphics[width=57mm]{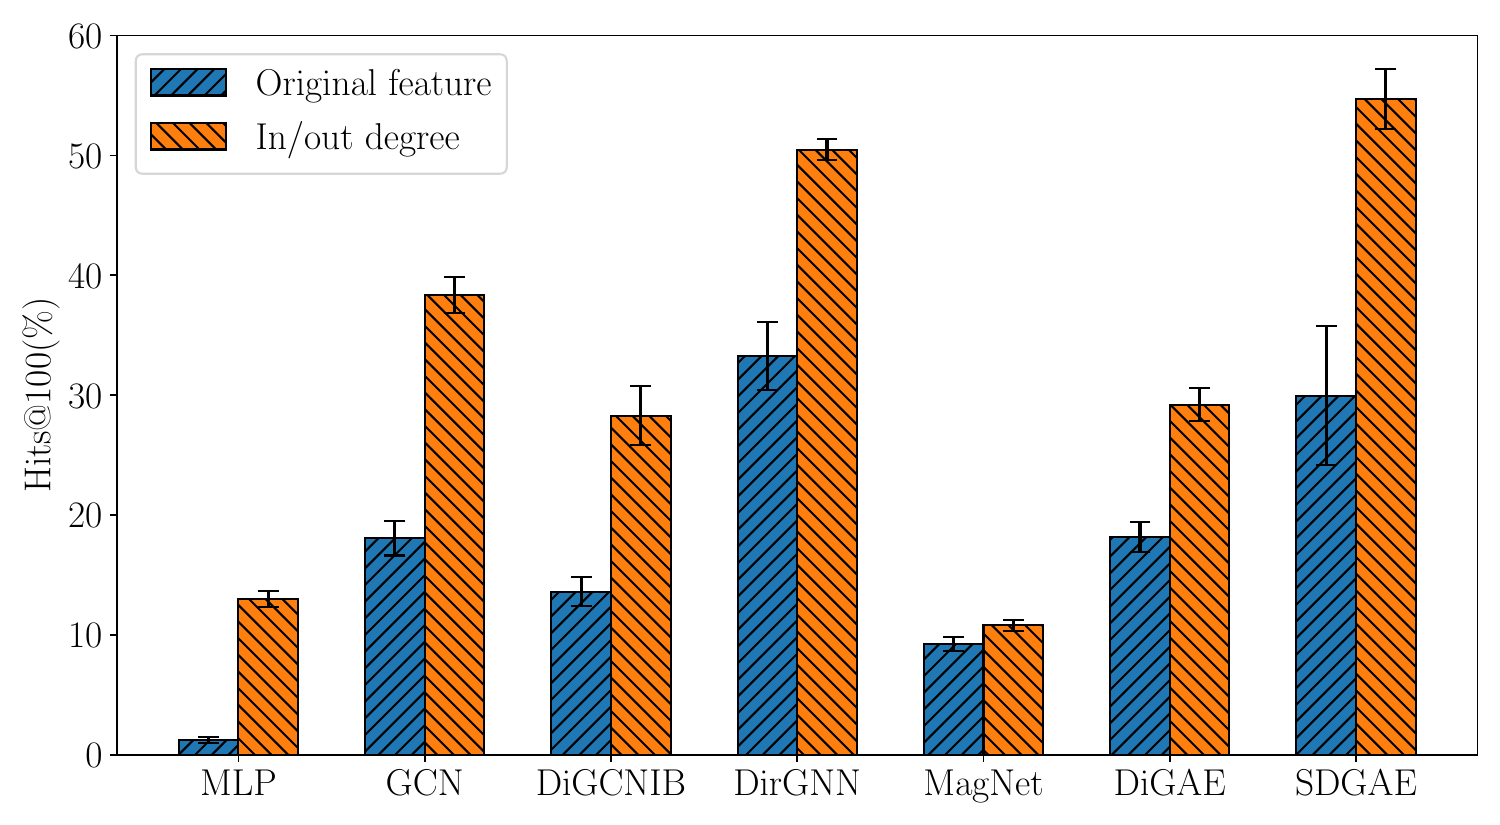}}
   \hspace{-4mm}
   \subfigure[Slashdot]{
   \label{fig:app_feature_slsh}
   \includegraphics[width=57mm]{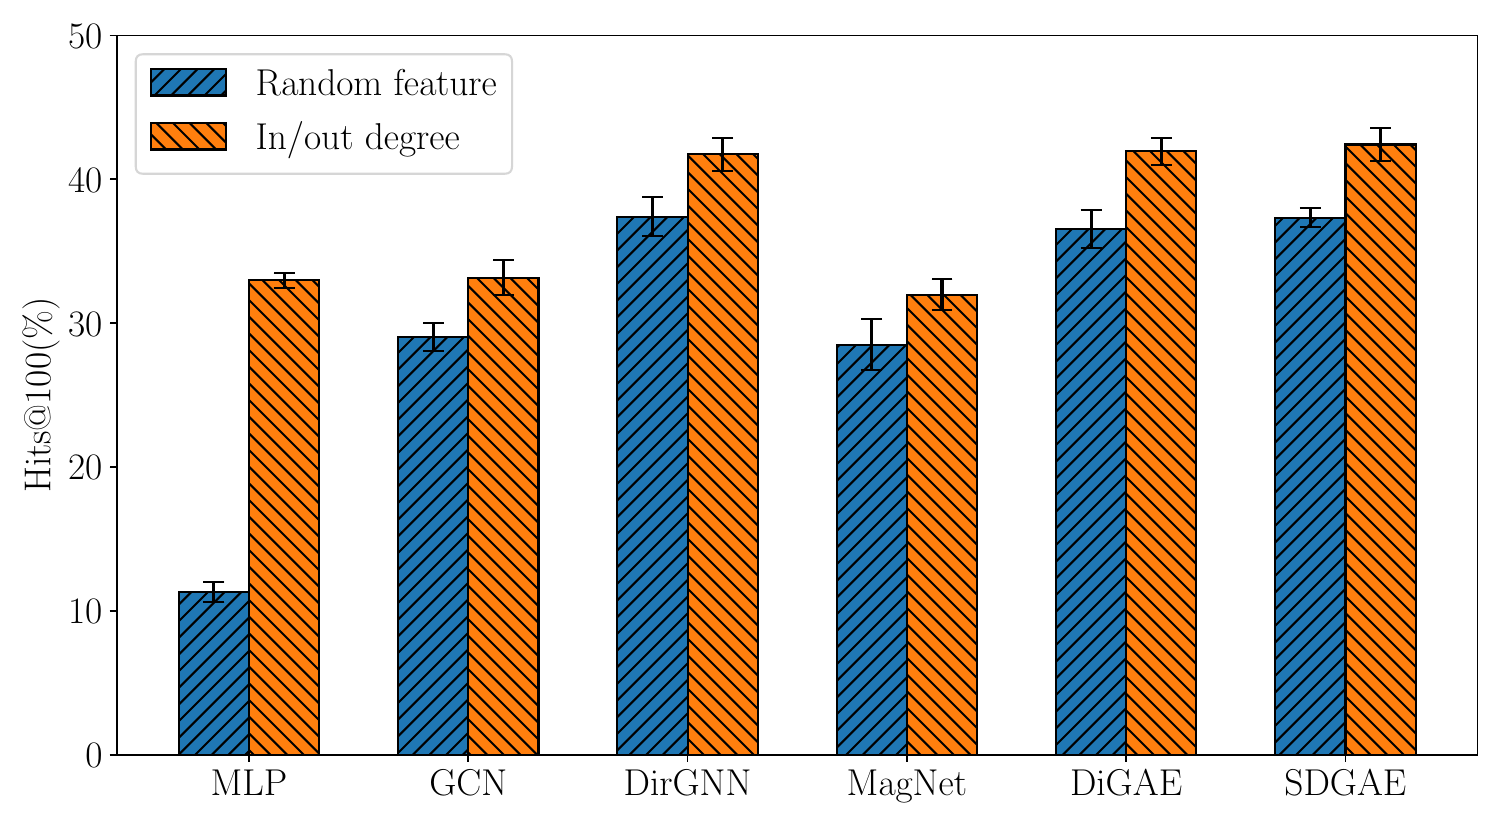}}
   \hspace{-4mm}
   \vspace{-2mm}
   \caption{Comparison of various methods' performance using original features, in/out degrees, or random features as inputs on 3 datasets.}
    \vspace{-2mm}
   \label{fig:app_feature}
\end{figure*}

\hypertarget{app_bench_res_ana}{}
\subsection{Additional results in analysis}
\label{app_bench_res_ana}

\subsubsection{Feture inputs}\label{app_feature_input}
In Figures~\ref{fig:app_feature_photo} and~\ref{fig:app_feature_wiki}, we compare the performance of various methods using original features and in/out degrees as inputs on Photo and WikiCS. Figure~\ref{fig:app_feature_slsh} presents a similar comparison using random features and in/out degrees as inputs on Slashdot. The results highlight the significant impact of feature inputs on GNN performance and also demonstrate that in-/out-degree information plays a crucial role in link prediction.

 \begin{figure}[ht]
    \centering
   \vspace{-1mm}
%   %\hspace{-3mm} 
    \subfigure[Cora-ML]{
   \includegraphics[width=72mm]{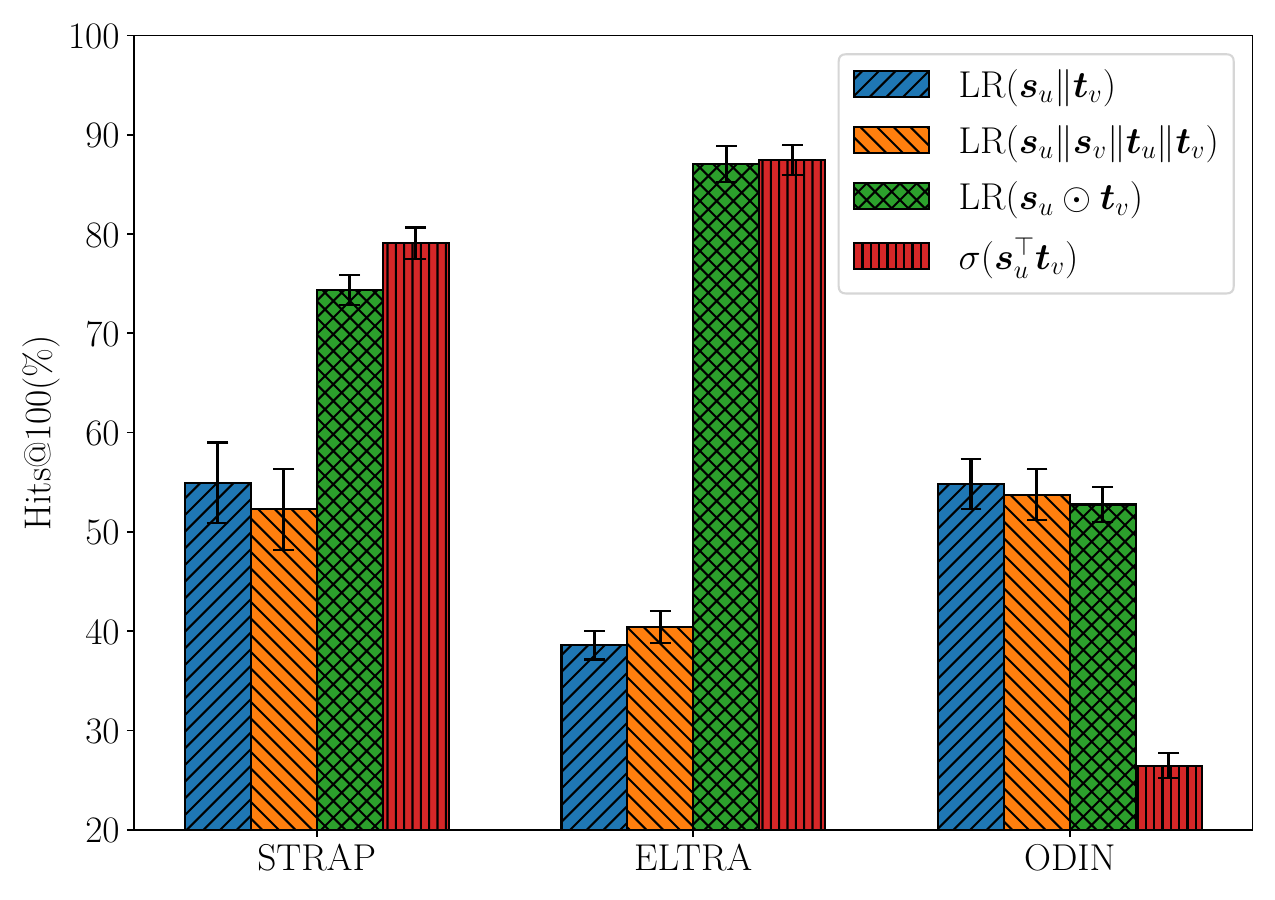}
   }
   \subfigure[Slashdot]{
   \includegraphics[width=72mm]{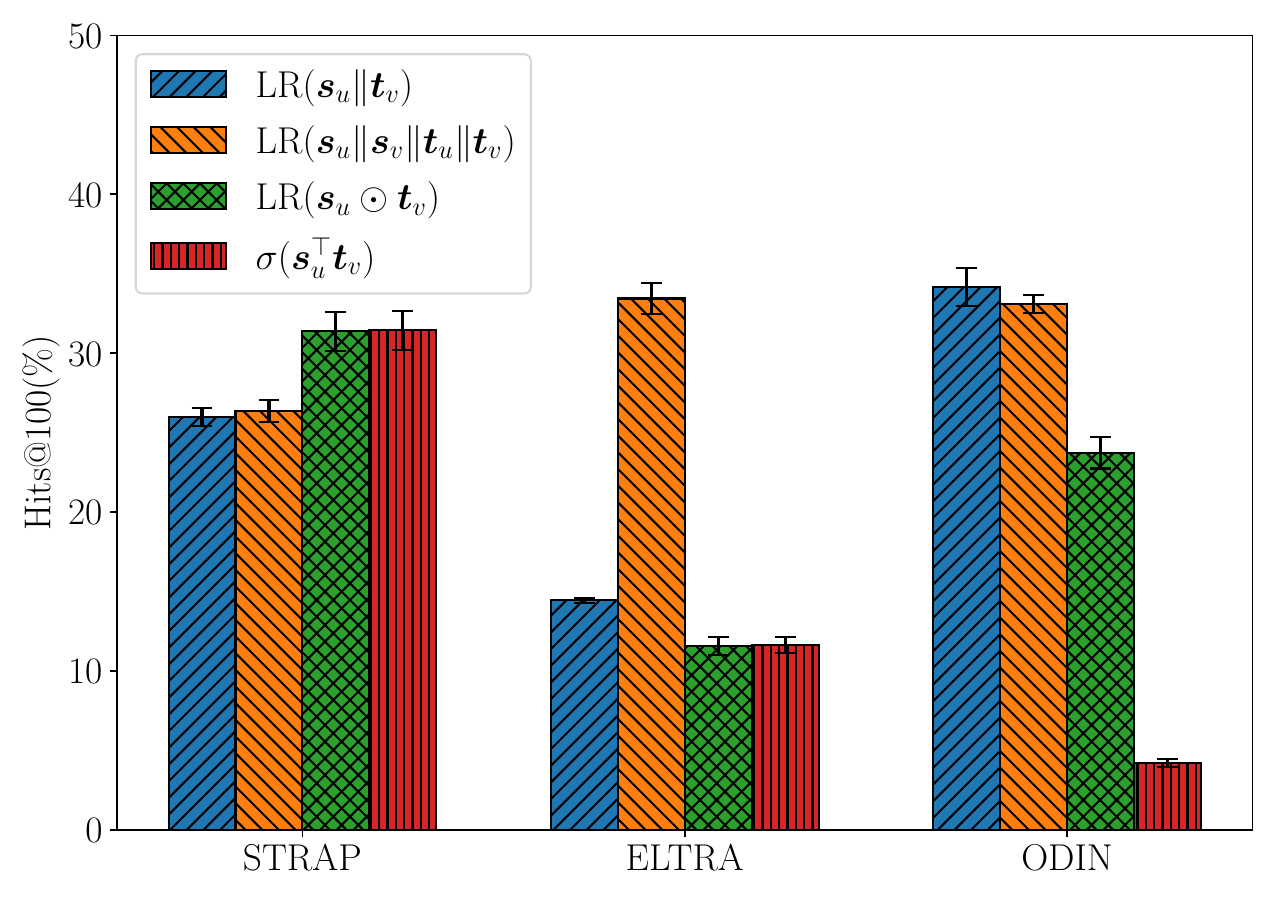}
   }
    \vspace{-2mm}
   \caption{Comparison of different decoders on embedding methods}
   \vspace{-1mm}
    \label{fig:app_loss_embedding}
 \end{figure}

 \begin{figure}[ht]
    \centering
   \vspace{-1mm}
%   %\hspace{-3mm} 
    \subfigure[Cora-ML]{
   \includegraphics[width=72mm]{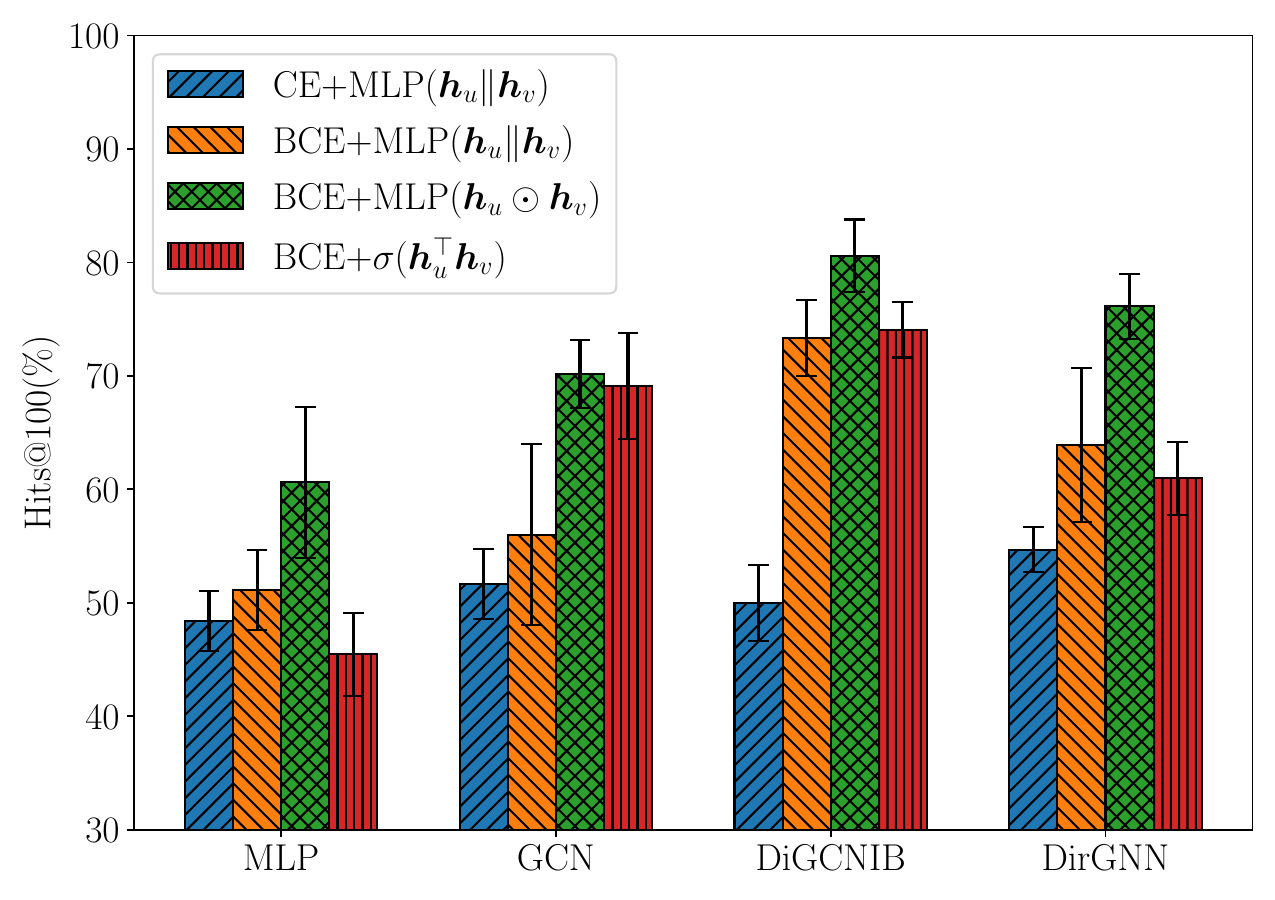}
   }
   \subfigure[Photo]{
   \includegraphics[width=72mm]{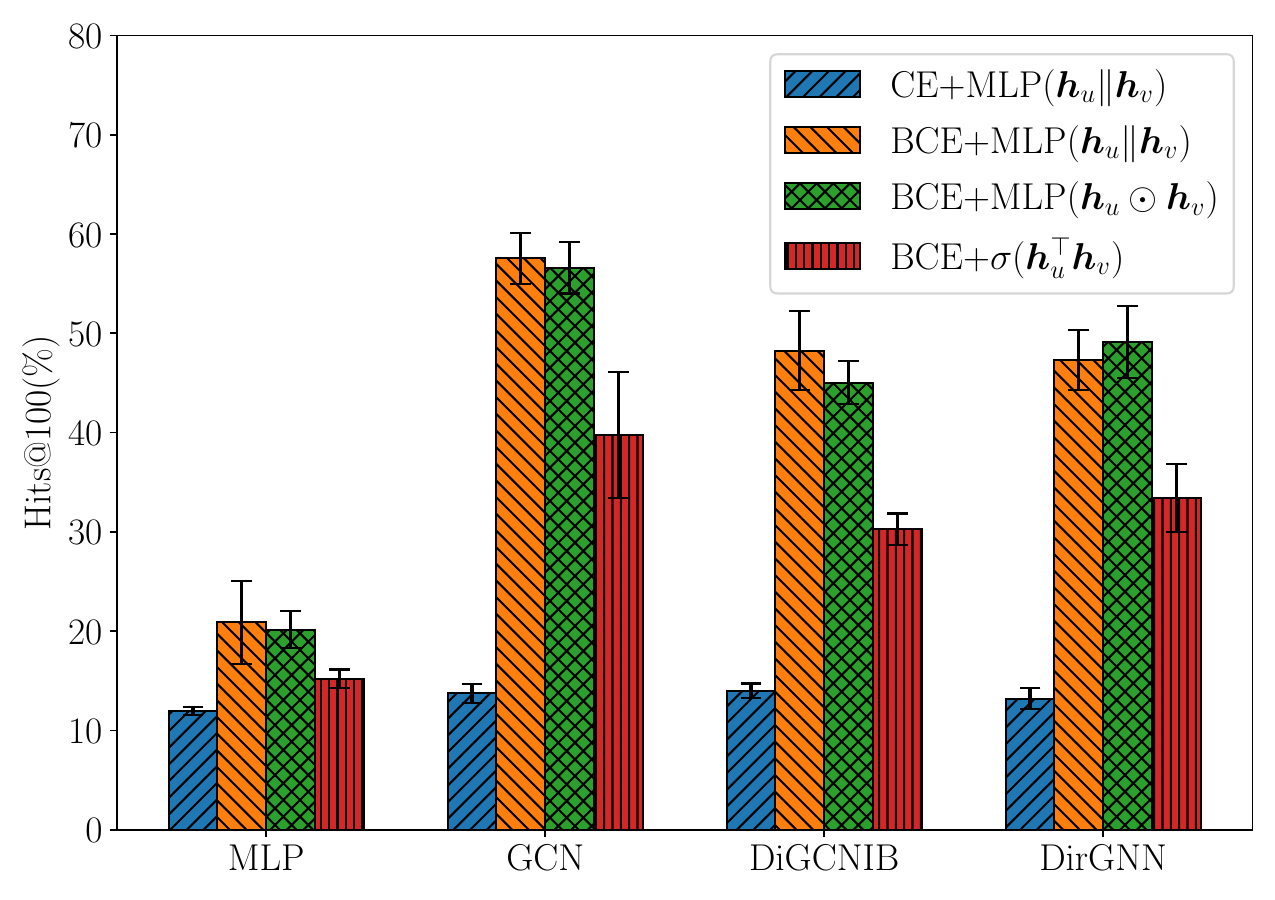}
   }
   \vspace{-2mm}
   \caption{Comparison of various loss functions with different decoders on GNNs.}
    \label{fig:app_loss_gnn}
 \end{figure}

\subsubsection{Loss function and decoder}\label{app_loss_function}
We present a comparison of different decoders on embedding methods in Figure~\ref{fig:app_loss_embedding} and a comparison of various loss functions with different decoders on GNNs in Figure~\ref{fig:app_loss_gnn}. These results highlight the significant impact of the loss function and decoder on the performance of directed link prediction methods. For embedding methods, even when using the same embeddings, different decoders can lead to substantial variations in performance. Notably, on the Slashdot dataset, ELTRA and ODIN are particularly sensitive to decoder settings. Furthermore, the results from GNNs on Cora-ML and Photo demonstrate that BCE loss provides a clear advantage. These findings emphasize the importance of carefully selecting loss functions and decoder configurations in link prediction tasks.

\begin{figure}[h]
\centering
   \vspace{-2mm}
   \hspace{-2mm}
   \subfigure{
   \includegraphics[width=37mm]{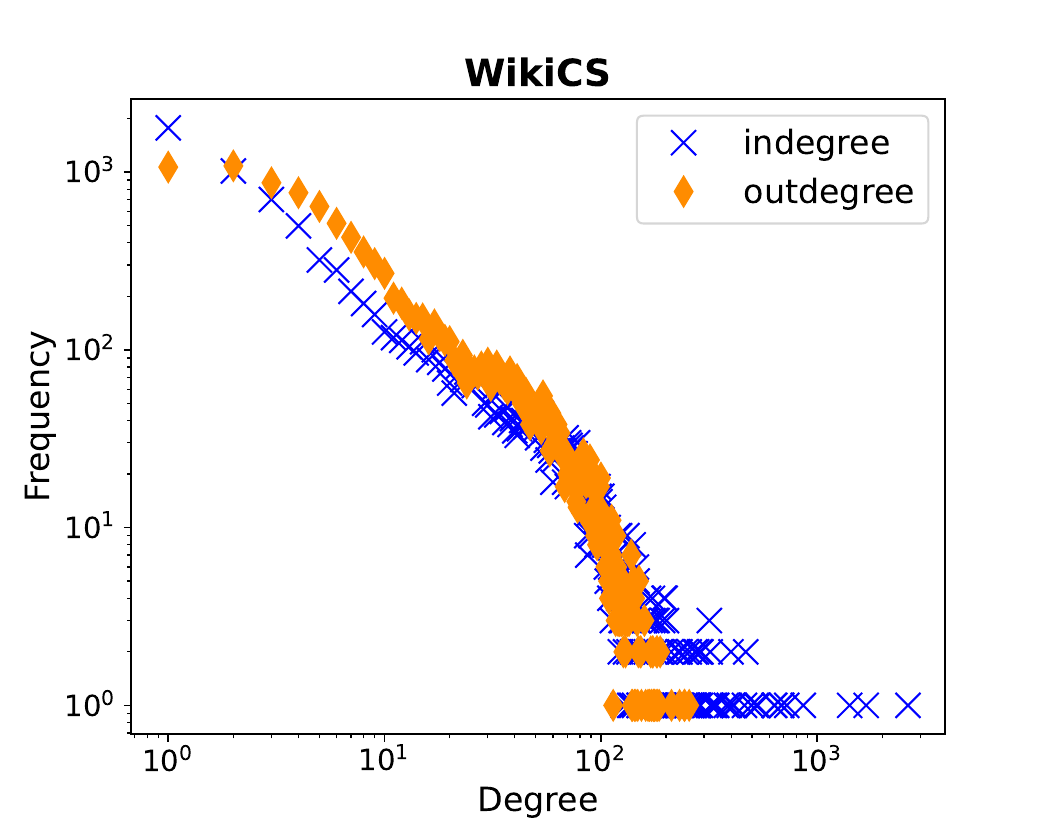}
   }
   \hspace{-7mm}
   \subfigure{
   \includegraphics[width=37mm]{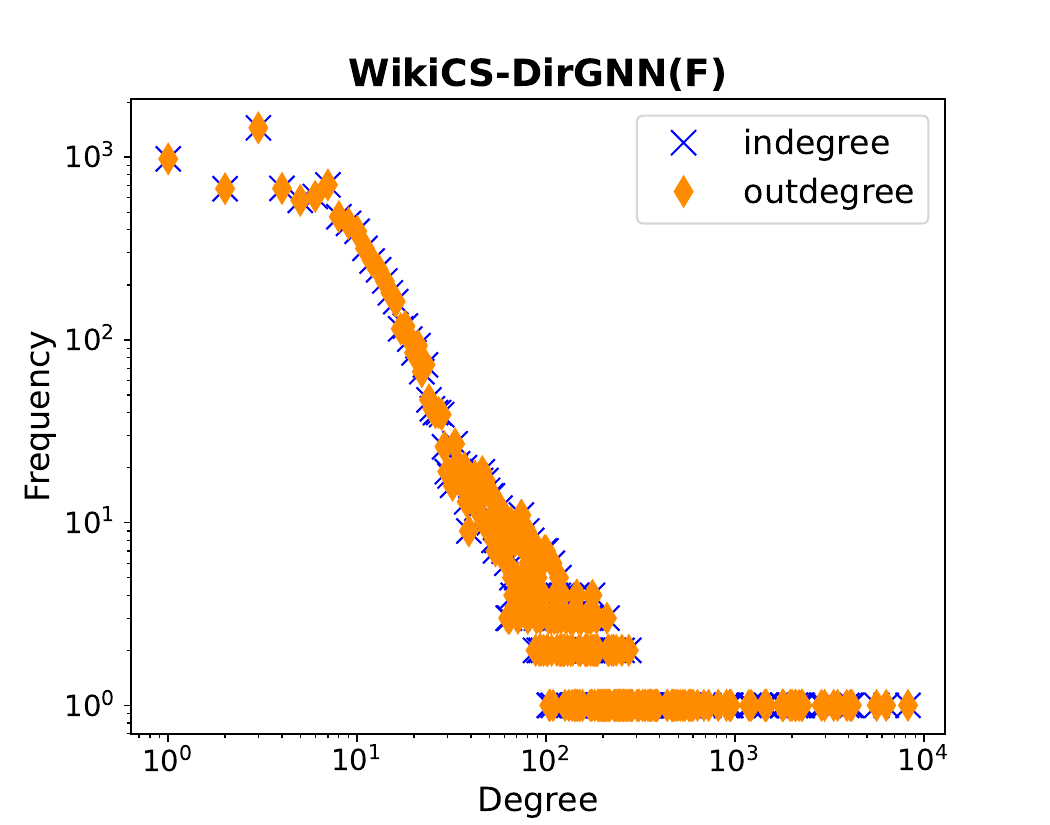}
   }
   \hspace{-7mm}
   \subfigure{
   \includegraphics[width=37mm]{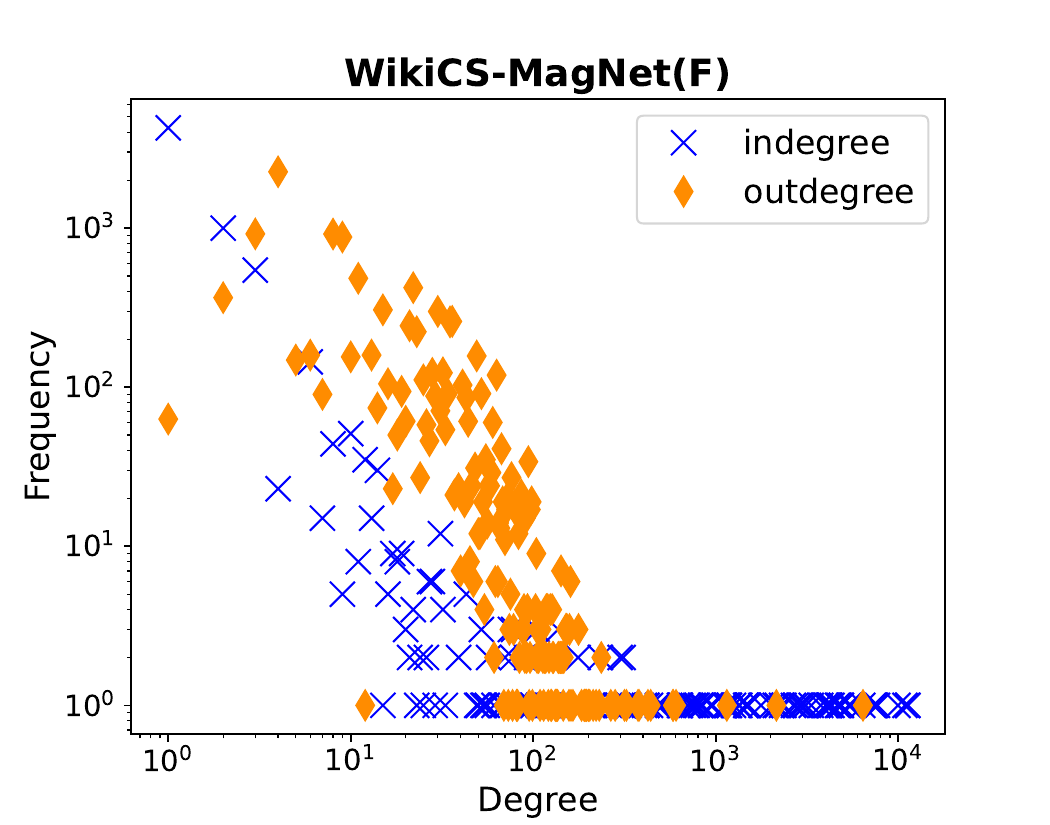}
   }
   \hspace{-7mm}
   \subfigure{
   \includegraphics[width=37mm]{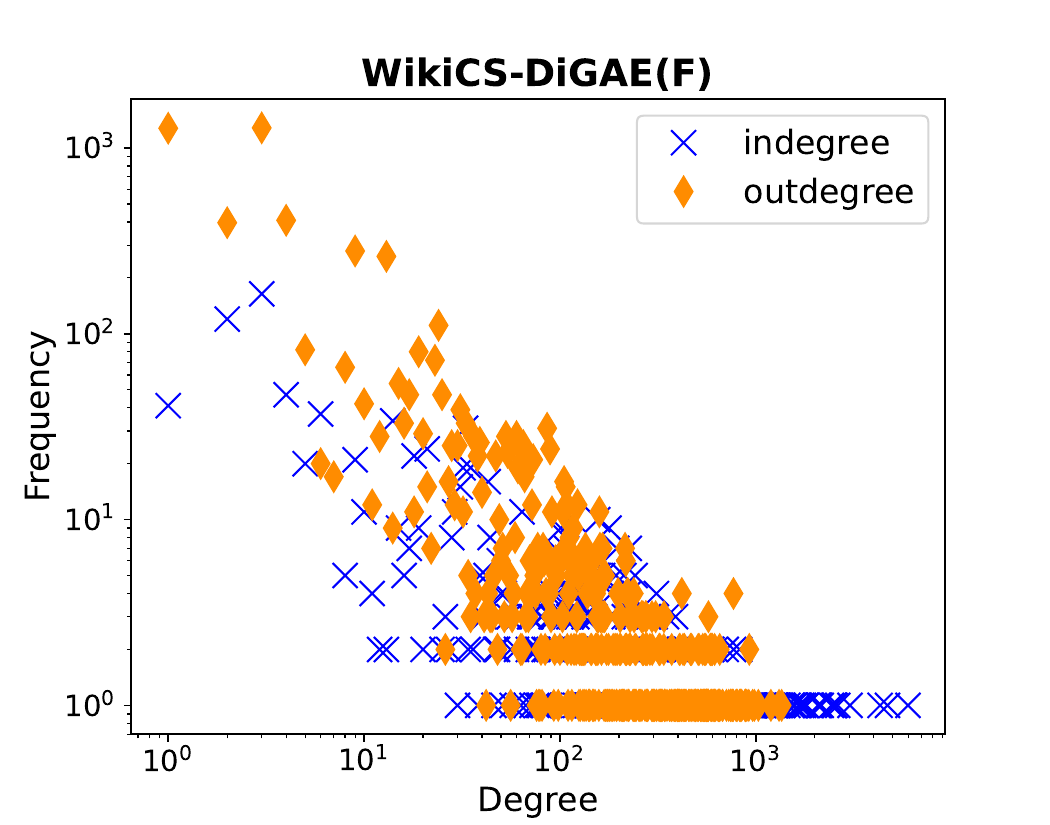}
   }
   \hspace{-7mm}
   \subfigure{
   \includegraphics[width=37mm]{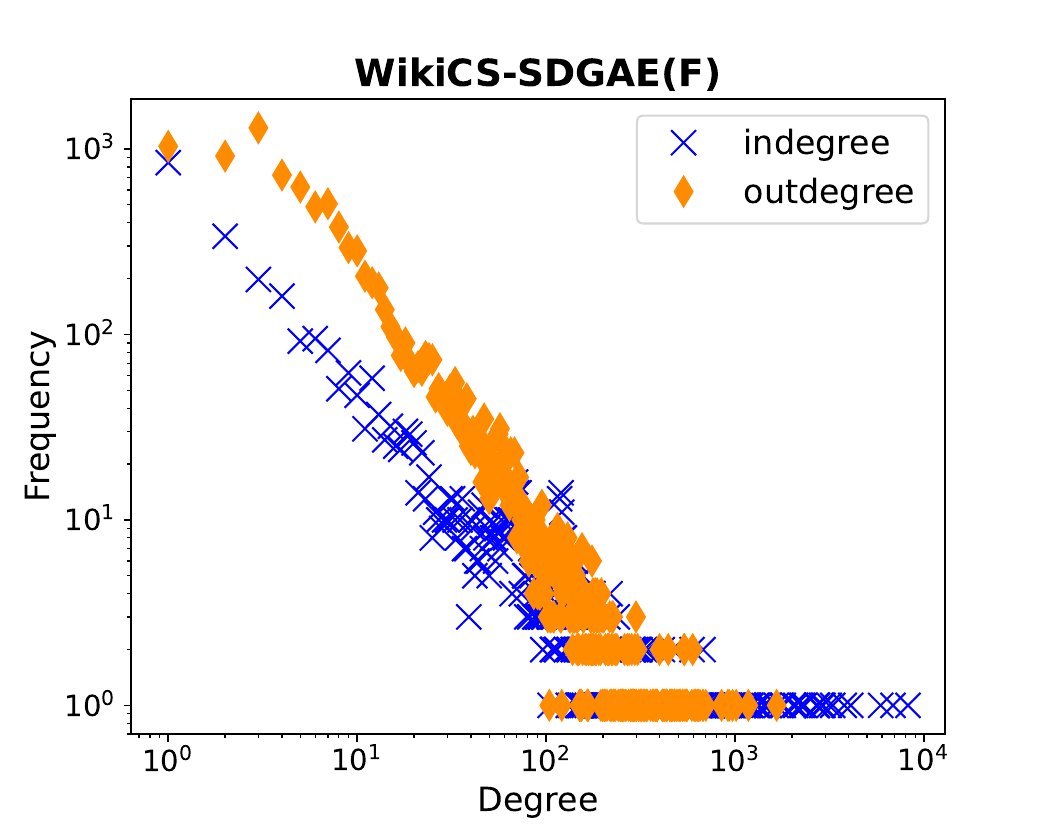}
   }
   \vspace{-5mm}
   \centering
   \caption{Degree distribution of WikiCS graph and its reconstruction graph generated by GNNs using the original feature as inputs.}
   %\vspace{-2mm}
   \label{fig:app_degree_feature}
\end{figure}

\begin{figure}[t]
    \centering
   \hspace{-3mm}
   \subfigure{
   \includegraphics[width=37mm]{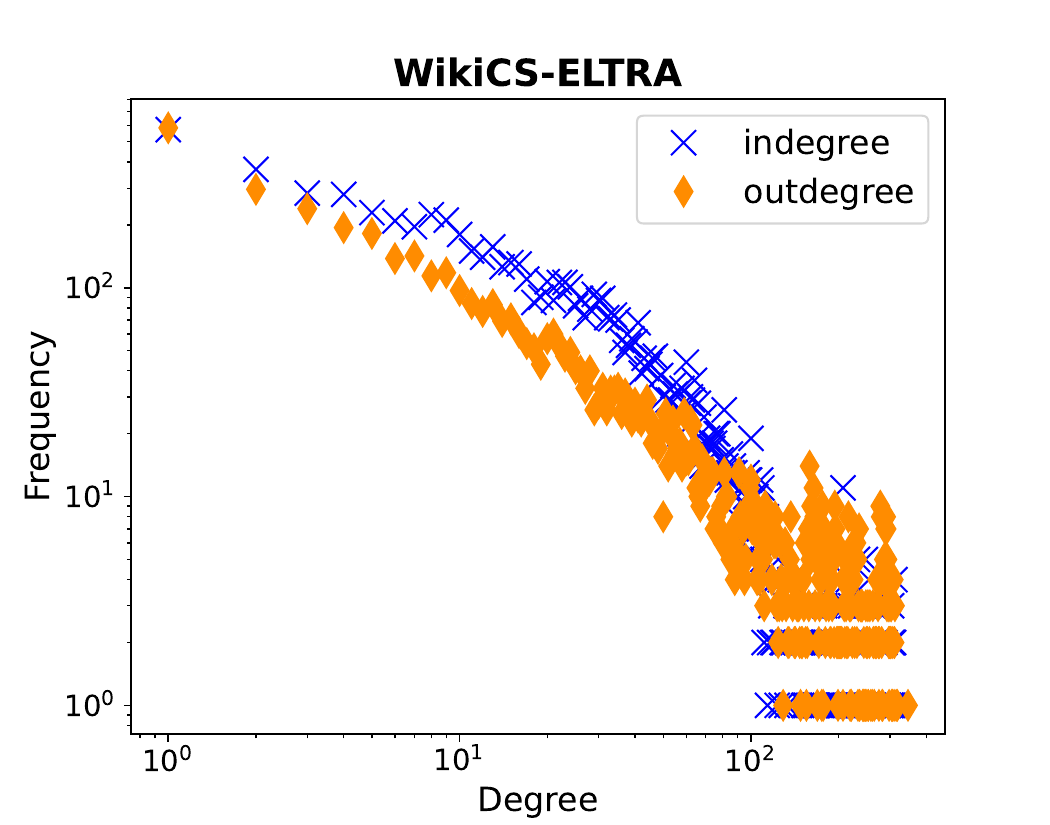}
   }
   \hspace{-7mm}
   \subfigure{
   \includegraphics[width=37mm]{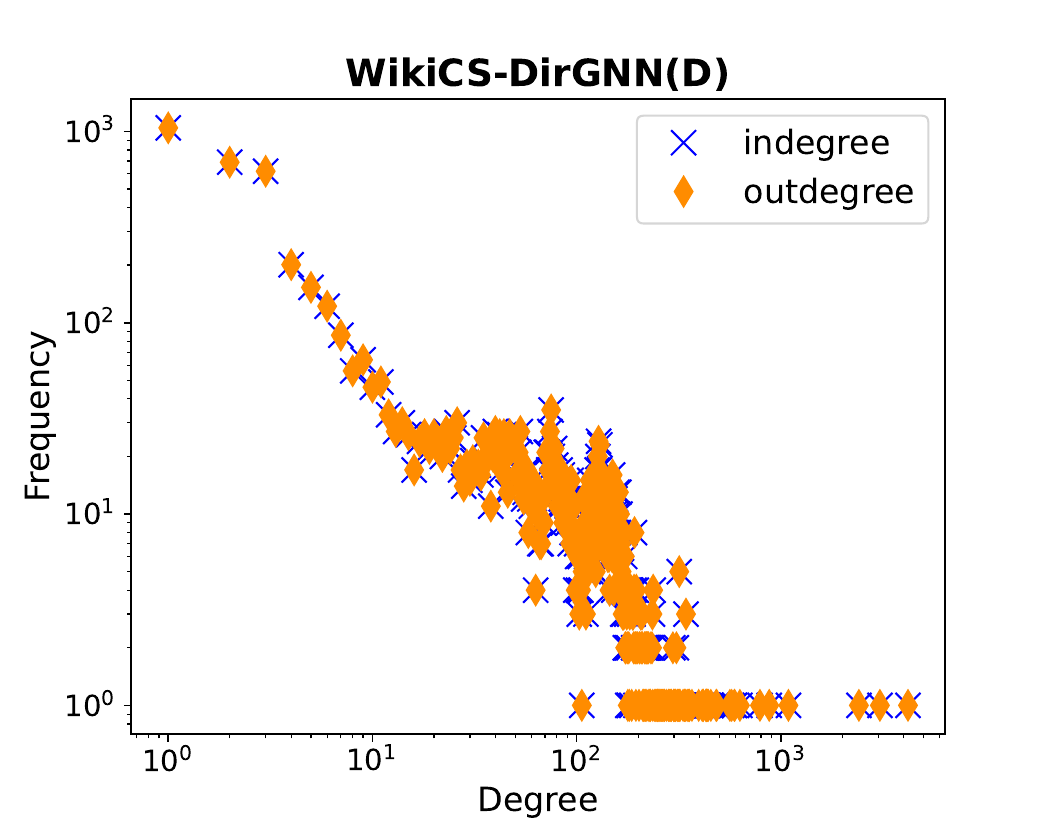}
   }
   \hspace{-7mm}
   \subfigure{
   \includegraphics[width=37mm]{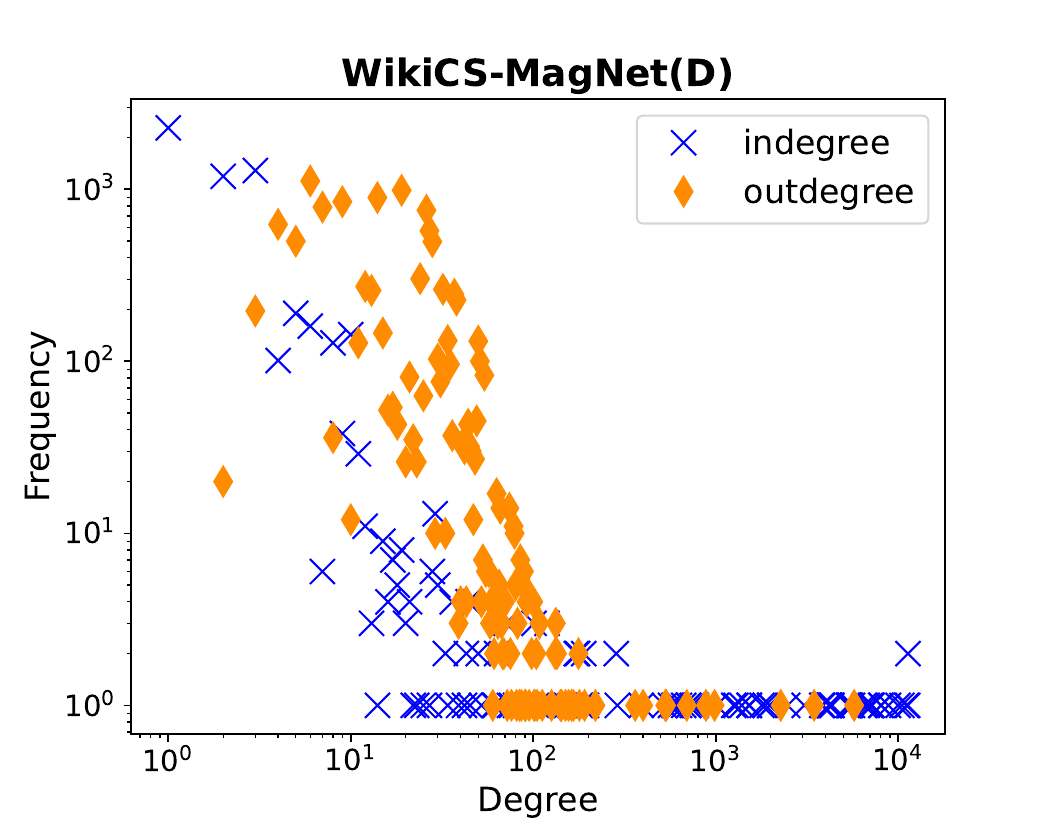}
   }
   \hspace{-7mm}
   \subfigure{
   \includegraphics[width=37mm]{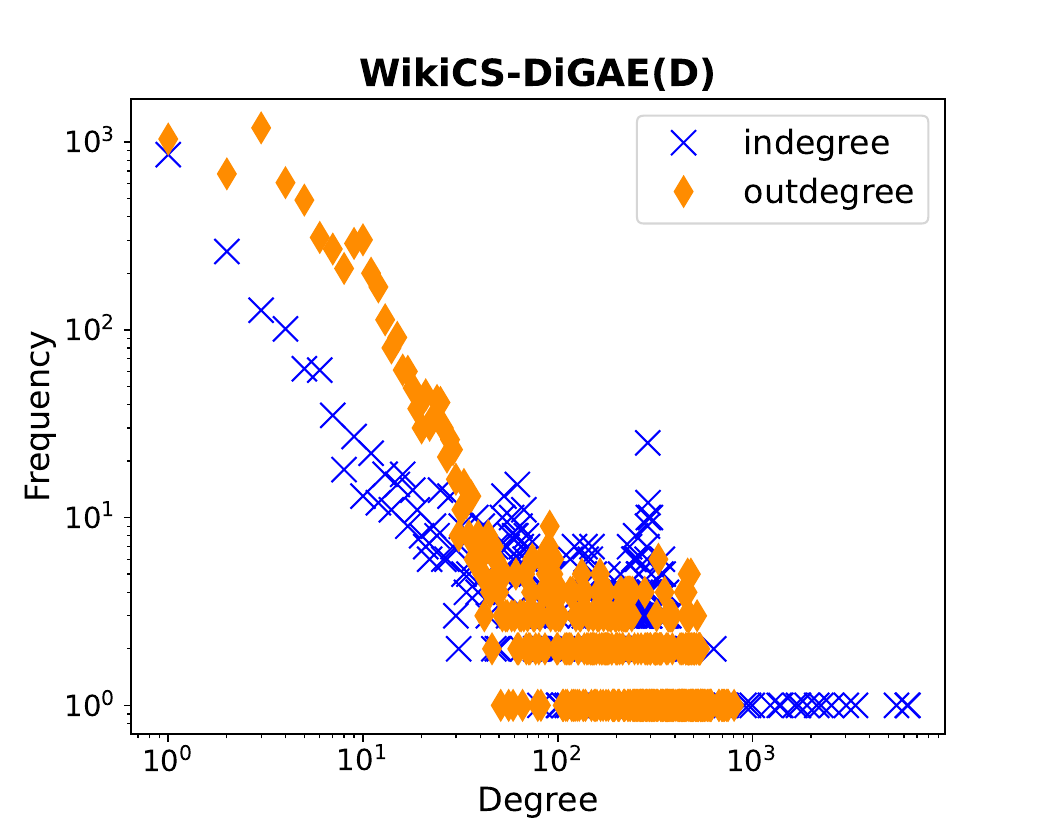}
   }
   \hspace{-7mm}
   \subfigure{
   \includegraphics[width=37mm]{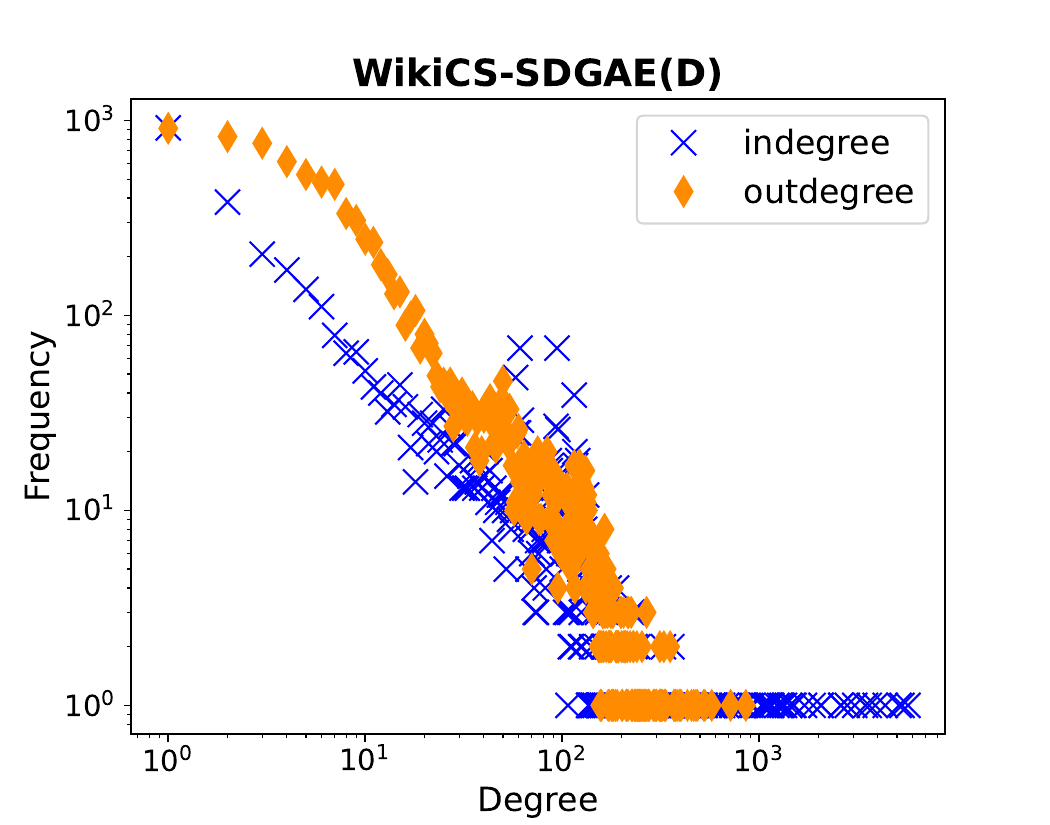}
   }
   \vspace{-3mm}
   \caption{Degree distribution of WikiCS's reconstruction graph generated by ELTRA and GNNs using the in/out degrees as inputs.}
    \label{fig:app_degree_degree}
\end{figure}

\subsubsection{Degree distribution}\label{app_degree}
We present the degree distribution of the WikiCS graph alongside its reconstructed versions generated by ELTRA and GNNs in Figures~\ref{fig:app_degree_feature} and~\ref{fig:app_degree_degree}. The GNNs use either the original features or the in/out degrees as inputs. First, we observe that ELTRA does not effectively preserve the degree distribution of WikiCS. This may be because ELTRA is primarily designed for directed graphs with many directed edges~\cite{eltra}, whereas WikiCS contains many undirected edges, which likely contributes to its poor performance on this dataset. Second, when GNNs use in/out degrees as inputs, they better preserve the degree distribution, which explains their improved performance on WikiCS for the link prediction task. This finding further underscores the importance of degree distribution in link prediction. Finally, comparing DiGAE and SDGAE, we find that SDGAE preserves the degree distribution more effectively, demonstrating the advantages of our proposed SDGAE.

\begin{table}[h]
\centering
\caption{The impact of normalization of adjacency matrix on DiGAE and SDGAE.}
\begin{tabular}{lcccc}
\toprule
Methods &Cora-ML	&CiteSeer	&Photo	&Computers  \\ \midrule
DiGAE ($\hat{\mD}_{\rm out}^{-\beta}\hat{\mA}\hat{\mD}_{\rm in}^{-\alpha}$) &82.06$\pm$2.51 	&83.64$\pm$3.21	&55.05$\pm$2.36	&41.55$\pm$1.62  \\
DiGAE ($\hat{\mD}_{\rm out}^{-1/2}\hat{\mA}\hat{\mD}_{\rm in}^{-1/2}$)&70.89$\pm$3.59	&71.60$\pm$6.21	&38.75$\pm$5.20	&32.73$\pm$5.28   \\
SDGAE ($\hat{\mD}_{\rm out}^{-1/2}\hat{\mA}\hat{\mD}_{\rm in}^{-1/2}$) &90.37$\pm$1.33	&93.69$\pm$3.68 	&68.84$\pm$2.35 	&53.79$\pm$1.56 \\
\bottomrule
\end{tabular}
\label{app_norm}
\end{table}

\subsubsection{SDGAE versus DiGAE}\label{app_sdgae_digae}
In Table~\ref{app_norm}, we compare the impact of different normalizations of the adjacency matrix on DiGAE and SDGAE. Here, $\hat{\mD}_{\rm out}^{-\beta}\hat{\mA}\hat{\mD}_{\rm in}^{-\alpha}$ represents the original settings in the DiGAE paper~\cite{digae}. We searched for the optimal parameters within the given range, $(\alpha,\beta) \in \{0.0, 0.2, 0.4, 0.6, 0.8\}^2$, noting that this does not include $\hat{\mD}_{\rm out}^{-1/2}\hat{\mA}\hat{\mD}_{\rm in}^{-1/2}$. As shown in Table~\ref{app_norm}, even when DiGAE uses $\hat{\mD}_{\rm out}^{-1/2}\hat{\mA}\hat{\mD}_{\rm in}^{-1/2}$, its performance did not improve. This indicates that SDGAE’s performance gains are not solely due to changes in the normalization of the adjacency matrix.

\begin{table}[h]
    \centering
    \caption{Comparison of negative sampling strategy on Cora-ML and CiteSeer datasets.}
    \resizebox{\textwidth}{!}{
    \begin{tabular}{llccccccc}
        \toprule
        Dataset & Sample & MLP & GCN & DiGCNIB & DirGNN & MagNet & DiGAE & SDGAE \\
        \midrule
        \multirow{2}{*}{Cora-ML} &each run& 60.61$\pm$6.64  & 70.15$\pm$3.01  & 80.57$\pm$3.21  & 76.13$\pm$2.85  & 56.54$\pm$2.95  & 82.06$\pm$2.51  & 90.37$\pm$1.33  \\
        & each epoch & 34.15$\pm$3.54  & 59.86$\pm$9.89  & 56.74$\pm$4.08  & 49.89$\pm$3.59  & 54.79$\pm$2.98  & 79.76$\pm$3.28  & 89.71$\pm$2.36  \\
        \midrule
        \multirow{2}{*}{CiteSeer} & each run  & 70.27$\pm$3.40  & 80.36$\pm$3.07  & 85.32$\pm$3.70  & 76.83$\pm$4.24  & 65.32$\pm$3.26  & 83.64$\pm$3.21  & 93.69$\pm$3.68  \\
        &  each epoch & 66.92$\pm$6.50  & 69.48$\pm$6.60  & 61.69$\pm$6.87  & 53.8$\pm$12.41  & 70.56$\pm$2.06  & 87.32$\pm$3.79  & 92.12$\pm$3.96  \\
        \bottomrule
    \end{tabular}}
    
    \label{app_sample}
\end{table}

\subsubsection{Metric and negative sampling strategy}\label{app_metrci_sampling}
We report the DirLinkBench results under the Accuracy metric in Table~\ref{tab:accuracy_performance} and compute the average rank and average score for each baseline. From these results, we observe that simple undirected graph GNNs can achieve competitive performance, with only a small gap between different methods. Notably, some methods that perform well under the Hits@100 metric (e.g., STRAP, DiGAE) perform relatively poorly in Accuracy. Additionally, in Appendix~\ref{app_complete_res}, we provide the complete DirLinkBench results for each metric across the seven datasets, including AUC, AP, and others. Analyzing these results, we find that AUC and AP exhibit minimal differentiation across baselines, making it difficult to accurately assess link prediction effectiveness. This aligns with ongoing discussions regarding the limitations of these metrics for evaluating link prediction tasks on undirected graphs~\cite{yang2015evaluating,li2023evaluating}. Therefore, we argue that ranking-based metrics, such as Hits@K and MRR, are more suitable for link prediction tasks.

We compare the impact of different negative sampling strategies on model performance during training in Table~\ref{app_sample}, presenting results for seven GNNs on Cora-ML and CiteSeer. Here, ``each run" refers to the default setting in DirLinkBench, where a random negative sample is generated for each run and shared across all models. In contrast, ``each epoch" represents a strategy where different models randomly sample negative edges in each training epoch. The positive sample splitting and test set remain consistent across comparisons. These results indicate that modifying the negative sampling strategy during training significantly affects model performance, particularly for single real-valued GNNs, where test performance drops substantially. These findings suggest that negative sampling strategies during training deserve further research. For instance, heuristic-based methods have been proposed as alternatives to random sampling in undirected graphs~\cite{li2023evaluating}, which could be explored in future work.

\begin{table*}[t]
    \centering
    \caption{Results of various methods under the \textbf{Accuracy} metric (mean ± standard error\%). Results ranked \hig{1}{first}, \hig{2}{second}, and \hig{3}{third} are highlighted. TO indicates methods that did not finish running within 24 hours, and OOM indicates methods that exceeded memory limits.}
    \label{tab:accuracy_performance}
    \resizebox{\textwidth}{!}{
    \begin{tabular}{
        lcccccccrr 
    }
        \toprule
        {Method} & {Cora-ML} & {CiteSeer} & {Photo} & {Computers} & {WikiCS} & {Slashdot} & {Epinions} & {\makecell{Avg.\\ Rank $\downarrow$}} & {\makecell{Avg.\\ Score $\uparrow$}} \\
        \midrule
        STRAP & 78.47$\pm$0.77 & 75.01$\pm$1.40 & 94.61$\pm$0.10 & 93.43$\pm$0.07 & \hig{1}{94.57$\pm$0.06} & 88.19$\pm$0.08 & 91.89$\pm$0.06 & 8.71 & 88.02 \\
        ODIN & 77.16$\pm$0.84 & 73.63$\pm$1.19 & 80.60$\pm$0.20 & 81.73$\pm$0.10 & 86.39$\pm$0.08 & 90.39$\pm$0.10 & 92.42$\pm$0.07 & 11.86 & 83.19 \\
        ELTRA & 85.40$\pm$0.45 & 80.86$\pm$1.15 & 91.84$\pm$0.12 & 89.30$\pm$0.15 & 85.73$\pm$0.28 & 88.11$\pm$0.11 & 90.40$\pm$0.13 & 9.57 & 87.38 \\ \midrule
        
        MLP & 81.32$\pm$2.41 & 74.81$\pm$1.32 & 88.31$\pm$0.50 & 85.33$\pm$0.57 & 84.65$\pm$0.22 & 89.62$\pm$0.11 & 92.56$\pm$0.45 & 11.14 & 85.23 \\ \midrule
        
        GCN & 82.82$\pm$0.86 & 79.47$\pm$1.73 & \hig{3}{95.90$\pm$0.18} & \hig{2}{95.69$\pm$0.13} & 89.85$\pm$0.35 & 89.75$\pm$0.17 & \hig{3}{94.17$\pm$0.08} & 5.50 & 89.66 \\
        GAT & \hig{3}{88.95$\pm$0.71} & 85.94$\pm$1.21 & \hig{1}{96.17$\pm$0.20} & \hig{1}{95.78$\pm$0.26} & 88.90$\pm$0.36 & 88.01$\pm$0.49 & 92.92$\pm$0.37 & \hig{2}{4.64} & \hig{2}{90.95} \\
        APPNP & \hig{2}{89.90$\pm$0.73} & \hig{3}{86.23$\pm$1.49} & 94.71$\pm$0.29 & 94.01$\pm$0.16 & 87.51$\pm$0.14 & 90.07$\pm$0.10 & \hig{2}{94.17$\pm$0.16} & 5.07 & \hig{3}{90.94} \\ \midrule
        
        DGCN & 80.26$\pm$0.69 & 74.83$\pm$1.46 & 95.27$\pm$0.94 & 95.22$\pm$0.20 & 90.13$\pm$0.37 & TO & TO & 9.43 & 87.14 \\
        DiGCN & 82.47$\pm$0.97 & 80.38$\pm$1.17 & 93.86$\pm$0.23 & 93.44$\pm$0.54 & 88.89$\pm$0.14 & TO & TO & 9.86 & 87.81 \\
        DiGCNIB & 87.25$\pm$0.58 & 85.98$\pm$1.19 & 95.05$\pm$0.27 & 94.61$\pm$0.31 & 90.72$\pm$0.10 & TO & TO & 7.14 & 90.72 \\
        DirGNN & 85.83$\pm$0.93 & 80.34$\pm$1.52 & 95.34$\pm$0.17 & 94.68$\pm$0.14 & \hig{3}{91.55$\pm$0.25} & \hig{2}{90.65$\pm$0.13} & 93.99$\pm$0.05 & \hig{3}{4.86} & 90.34 \\ \midrule
        
        MagNet & 77.51$\pm$0.92 & 73.73$\pm$1.30 & 80.16$\pm$0.23 & 81.43$\pm$0.08 & 86.59$\pm$0.06 & \hig{3}{90.45$\pm$0.09} & 92.92$\pm$0.05 & 11.21 & 83.26 \\
        DUPLEX & 82.28$\pm$0.93 & 79.20$\pm$1.79 & 87.68$\pm$0.52 & 85.65$\pm$0.27 & 83.82$\pm$0.23 & 85.42$\pm$3.42 & 88.20$\pm$3.86 & 12.14 & 84.61 \\ \midrule
        
        DHYPR & 86.04$\pm$0.66 & \hig{2}{87.33$\pm$1.39} & 76.94$\pm$0.63 & TO & TO & OOM/TO & OOM/TO & 11.71 & 83.44 \\
        DiGAE & 86.25$\pm$0.80 & 81.85$\pm$1.31 & 91.77$\pm$0.18 & 89.52$\pm$0.15 & 82.53$\pm$0.48 & 85.67$\pm$0.28 & 90.17$\pm$0.14 & 9.86 & 86.82 \\ \midrule
        
        SDGAE & \hig{1}{91.36$\pm$0.70} & \hig{1}{91.38$\pm$0.79} & \hig{2}{96.16$\pm$0.14} & \hig{3}{95.66$\pm$0.12} & \hig{2}{92.24$\pm$0.12} & \hig{1}{91.05$\pm$0.20} & \hig{1}{94.33$\pm$0.11} & \hig{1}{1.57} & \hig{1}{93.17} \\
        \bottomrule
    \end{tabular}}
\end{table*}

%\subsection{Link prediction on directed graph problem}

%\textbf{Loss Function} Binary Cross-Entropy Loss (BCE-Loss) and Cross-Entropy Loss (CE-Loss).

%\begin{table*}[th]
%\centering
%\caption{The results on the DUPLEX's setting.}
%\resizebox{\textwidth}{!}{
%\begin{tabular}{@{}llllllll@{}}
%\toprule
%\multicolumn{1}{l}{Dataset}              & Method & EP(ACC) & EP(AUC) & DP(ACC)  & DP(AUC) & 3C(ACC) & 4C(ACC) \\ \midrule
%\multirow{3}{*}{CiteSeer} & DUPLEX (original) &95.7±0.5 &98.6±0.4 &98.7±0.4 &99.7±0.2 &94.8±0.2 &91.1±1.0 \\ %\cmidrule(l){2-7} 
%& DUPLEX (reproduced) &92.11±0.78 &95.85±0.87 &97.54±0.54 &98.93±0.59  &88.22±1.06 &84.77±1.01           \\
%                                      & MLP             \\ \midrule
%\multirow{3}{*}{Cora} & DUPLEX (original) &93.2±0.1 &95.9±0.1 &95.9±0.1 &97.9±0.2 &92.2±0.1 &88.4±0.4    \\
%& DUPLEX (reproduced) &93.49±0.21 &95.61±0.20 &95.25±0.16 &96.34±0.23  &92.41±0.21 &89.76±0.25     \\
%                                      & MLP             \\ \bottomrule
%\end{tabular}}
%\end{table*}

%\begin{figure}[ht]
%    \centering
%   \vspace{-1mm}
%   %\hspace{-3mm}  
%   \includegraphics[width=80mm]{figure/feature_cora.pdf}
%   \caption{Cora-ml.}
%   \vspace{-1mm}
    %\label{fig:duplex_cls_citeseer}
% \end{figure}
