# Supplementary material for: Rethinking Link Prediction for Directed Graphs
Source: arXiv:2502.05724 source file (2025-05-21)
Supplement: Supplementary file 3 [file appendix_issues.tex]

\hypertarget{app_issues}{} 
\section{Issues with Existing Experimental Setup}\label{app_issues}

\hypertarget{app_issues_subtask}{} 
\subsection{Details of multiple subtask setup}\label{app_issues_subtask}
The multiple subtask setup~\cite{magnet,dpyg,duplex} involves four subtasks where graph edges are categorized into four types: positive (original direction), reverse (inverse direction), bidirectional (both directions), and nonexistent (no connection). Each subtask focuses on predicting a specific edge type. The details are as follows:
\begin{itemize}[topsep=0pt, partopsep=0pt]
    \item Existence Prediction (EP): The model predicts whether a directed edge $(u, v)$ exists in the graph. Both reverse and nonexistent edges are treated as nonexistence.
    \item Directed Prediction (DP): The model predicts the direction of edges for node pairs $(u, v)$, where either $(u, v) \in E$ or $(v, u) \in E$.
    \item Three-Type Classification (3C): The model classifies an edge as positive, reverse, or nonexistent.
    \item Four-Type Classification (4C): The model classifies edges into four categories: positive, reverse, bidirectional, or nonexistent.
\end{itemize}

\begin{table}[h]
\centering
\caption{The results of MagNet~\cite{magnet} as reported in the original paper, alongside the reproduced MagNet and
MLP results.}
%\resizebox{\textwidth}{!}{
\begin{tabular}{@{}cllllll@{}}
\toprule
\multicolumn{1}{l}{Task}              & Method & Cornell & Texas & Wisconsin & Cora-ML & CiteSeer \\ \midrule
\multirow{3}{*}{DP} & MagNet (reported) &82.9$\pm$3.5 &80.9$\pm$4.2 &83.3$\pm$3.0 &86.5$\pm$0.7 &84.8$\pm$1.2 \\ %\cmidrule(l){2-7} 
                                      & MagNet (reproduced) &84.69$\pm$2.86 &87.15$\pm$4.49 &85.72$\pm$4.24 &\textbf{88.56$\pm$0.44}
                                      &\textbf{89.72$\pm$1.06}         \\
                                      & MLP    &\textbf{84.95$\pm$3.10} &\textbf{89.79$\pm$4.06} &\textbf{87.21$\pm$2.48}
                                      &86.56$\pm$0.70        &88.92$\pm$0.56          \\ \midrule
\multirow{3}{*}{EP} & MagNet (reported) &\textbf{81.1$\pm$3.3} &83.6$\pm$2.7 &\textbf{82.8$\pm$2.2} &\textbf{82.7$\pm$0.7} &79.9$\pm$0.6   \\
                                      & MagNet (reproduced)    
&75.42$\pm$6.25 &\textbf{84.52$\pm$4.12} &78.16$\pm$3.83 &80.04$\pm$0.89 &83.95$\pm$0.35\\
                                      & MLP       &76.01$\pm$4.64&82.97$\pm$4.33 &79.79$\pm$2.71 &79.47$\pm$1.08        &\textbf{84.78$\pm$0.56}          \\ \bottomrule
\end{tabular}
\label{tb_magnet}
\end{table}

\begin{table}[h]
\centering
\caption{The results of MLP and baselines under PyGSD~\cite{dpyg} setup on Direction Prediction (DP) task.}
%\resizebox{\textwidth}{!}{
\begin{tabular}{lcccccc}
\toprule
Method & Cora-ML & CiteSeer & Telegram & Cornell & Texas & Wisconsin \\ \midrule
MLP       &86.13$\pm$0.45  & 85.51$\pm$0.63  & 95.61$\pm$0.15  & \textbf{86.40$\pm$2.60}  &\textbf{83.08$\pm$4.33}  & \textbf{87.95$\pm$2.65}  \\ \midrule
DGCN      & 85.49$\pm$0.75  & 84.85$\pm$0.56  & 96.03$\pm$0.35  & 84.55$\pm$3.71  & 79.59$\pm$5.09  & 84.57$\pm$3.59  \\ 
DiGCN     & 85.37$\pm$0.54  & 83.88$\pm$0.82  & 94.95$\pm$0.54  & 85.41$\pm$2.78  & 76.57$\pm$3.98  & 82.41$\pm$2.56  \\ 
DiGCNIB   & 86.12$\pm$0.42  & 85.58$\pm$0.56  & 95.99$\pm$0.44  & 86.28$\pm$3.37  &82.27$\pm$3.51  &87.07$\pm$2.16  \\ 
MagNet    & \textbf{86.33$\pm$0.54}  & \textbf{85.80$\pm$0.63}  & \textbf{96.97$\pm$0.21}  & 83.29$\pm$4.28  & 80.25$\pm$4.78  & 86.60$\pm$2.72  \\ \bottomrule
\end{tabular}%}
\label{tb_dpyg_dp}
\end{table}

\begin{table}[h]
\centering
\caption{The results of MLP and baselines under PyGSD~\cite{dpyg} setup on Existence Prediction (EP) task.}
%\resizebox{\textwidth}{!}{
\begin{tabular}{lcccccc}
\toprule
Method & Cora-ML & CiteSeer & Telegram & Cornell & Texas & Wisconsin \\ \midrule
MLP       & \textbf{78.85$\pm$0.83}  & 71.03$\pm$0.89  & 82.72$\pm$0.57  & 68.41$\pm$2.05  & \textbf{69.58$\pm$2.29}  & \textbf{72.53$\pm$2.27}  \\ \midrule 
DGCN      & 76.45$\pm$0.49  & 70.72$\pm$0.79  & 83.18$\pm$1.55  & 67.95$\pm$2.27  & 63.65$\pm$2.40  & 68.12$\pm$2.86    \\ 
DiGCN     & 76.17$\pm$0.49  & 72.00$\pm$0.88  & 83.12$\pm$0.43  & 67.16$\pm$1.82  & 63.54$\pm$3.85  & 67.01$\pm$2.47    \\ 
DiGCNIB   & 78.80$\pm$0.51  & \textbf{74.55$\pm$0.91}  & 84.49$\pm$0.51  & \textbf{69.77$\pm$2.05}  & 67.60$\pm$3.44  & 70.78$\pm$2.79   \\ 
MagNet    & 77.37$\pm$0.45  & 71.47$\pm$0.71  & \textbf{85.82$\pm$0.39}  & 68.98$\pm$2.27  & 65.94$\pm$1.88  & 71.23$\pm$2.53    \\  \bottomrule
\end{tabular}%}
\label{tb_dpyg_ep}
\end{table}

\hypertarget{app_issues_results}{} 
\subsection{Details of experimental setting and more results}\label{app_issues_results}
\textbf{Experimental setting}. In this part of the experiment, we strictly follow the configurations of each setup and reproduce the results using the provided codes. For the MLP model, we implement a simple two-layer network with 64 hidden units, while the learning rate and weight decay are tuned according to the settings of each setup to ensure a fair comparison. For the MagNet~\cite{magnet} setup, we reproduce the reported MagNet results and include the MLP results. For PyGSD~\cite{dpyg} setup, we get the results in our environment using their baseline code and settings, and report the MLP results. For DUPLEX~\cite{duplex}, we reproduce the DUPLEX results and additionally report the results of graph propagation without using the test edges and the MLP results.

%PyGSD is a software package designed for Signed and Directed Graphs, built on PyTorch Geometric (PyG). 

\begin{table}[h]
\centering
\caption{Link prediction results for CiteSeer dataset under the DUPLEX~\cite{duplex} setup: no superscripts are from the DUPLEX paper, $^\dagger$ indicates reproduction with test set edges in training, and $^\ddagger$ indicates reproduction without test set edges in training.}
%\resizebox{\textwidth}{!}{
\begin{tabular}{@{}lllllll@{}}
\toprule

%\multicolumn{1}{l}{\multirow{2}{*}{Dataset}} & \multirow{2}{*}{Method} & \multicolumn{2}{c}{EP} & \multicolumn{2}{c}{DP} & 3C  & 4C  \\ \cmidrule(l){3-8} 
Method &EP(ACC) &EP(AUC) &DP(ACC) &DP(AUC) &3C(ACC) &4C(ACC) \\ \midrule
%\multicolumn{1}{l}{} & & ACC  & AUC  & ACC   & AUC  & ACC & ACC \\ \midrule

MagNet &80.7$\pm$0.8 &88.3$\pm$0.4 &91.7$\pm$0.9 &96.4$\pm$0.6 &72.0$\pm$0.9 &69.3$\pm$0.4 \\ 
DUPLEX &95.7$\pm$0.5 &98.6$\pm$0.4 &98.7$\pm$0.4 &99.7$\pm$0.2 &94.8$\pm$0.2 &91.1$\pm$1.0  \\ \midrule

DUPLEX$^\dagger$ &92.11$\pm$0.78 &95.85$\pm$0.87 &97.54$\pm$0.54 &98.93$\pm$0.59  &88.22$\pm$1.06 &84.77$\pm$1.01 \\
MLP$^\dagger$ &85.74$\pm$1.80	&93.33$\pm$1.27	&\textbf{97.55$\pm$0.97}	&\textbf{99.58$\pm$0.52}	&81.20$\pm$0.82	&76.30$\pm$0.62  \\ \midrule 

DUPLEX$^\ddagger$  &83.59$\pm$1.47 &89.34$\pm$1.03 &85.56$\pm$1.36 &91.82$\pm$0.98 &76.37$\pm$2.07 &73.80$\pm$2.01 \\
MLP$^\ddagger$ &77.34$\pm$1.86	&87.36$\pm$1.26	&\textbf{89.19$\pm$0.95}	&\textbf{95.97$\pm$0.61}	&67.82$\pm$1.21	&64.25$\pm$1.35 \\ \bottomrule

\end{tabular}
\label{tb:app_duplex}
\end{table}

\textbf{Results with the MagNet setup}. Table~\ref{tb_magnet} presents the results of MagNet~\cite{magnet} as reported in the original paper, alongside the reproduced MagNet and MLP results, with the highest values bolded for emphasis. These results directly correspond to Figures~\ref{fig:dp} and~\ref{fig:ep}.

\begin{wrapfigure}{r}{0.45\textwidth} % 右侧浮动，占 45% 宽度
    \centering
    \vspace{-3mm}
    \includegraphics[width=\linewidth]{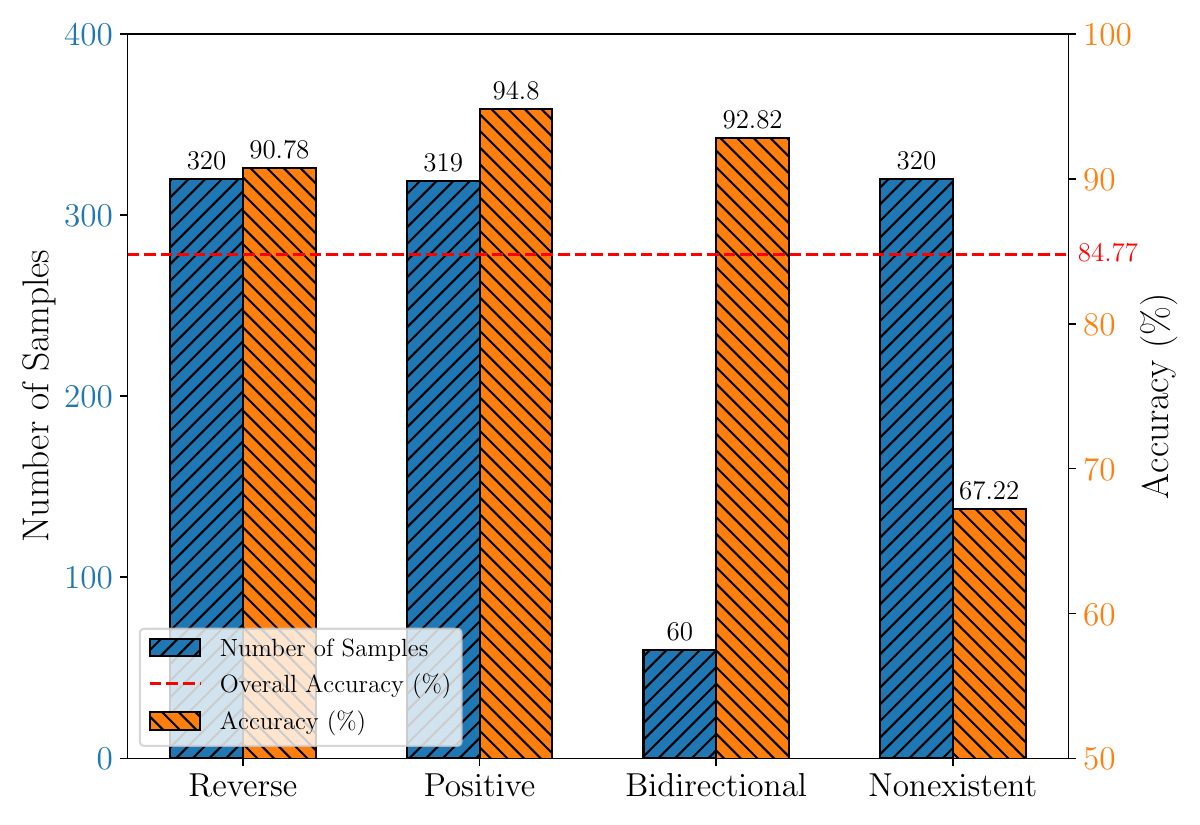}
    \vspace{-8mm}
    \caption{The number of samples and accuracy for each class of DUPLEX on the CiteSeer dataset in the 4C task.}
    \vspace{-2mm}
    \label{fig:duplex_cls_citeseer}
\end{wrapfigure}

\textbf{Results with the PyGSD setup}. PyGSD~\cite{dpyg} is a software package for Signed and Directed Graphs, built on PyTorch Geometric (PyG)~\cite{pyg}. Tables~\ref{tb_dpyg_dp} and~\ref{tb_dpyg_ep} present the results of MLP alongside several baselines on the Direction Prediction (DP) and Existence Prediction (EP) tasks, with the highest values highlighted in bold. The baselines include DGCN~\cite{dgcn-tong}, DiGCN~\cite{digcn}, DiGCNIB~\cite{digcn}, and MagNet~\cite{magnet}, as used in PyGSD. Across six datasets, MLP demonstrates competitive performance, achieving state-of-the-art results for both tasks on the Texas and Wisconsin datasets.

\textbf{Results with the DUPLEX setup}. In Table~\ref{tb:app_duplex}, we present the link prediction results for the CiteSeer dataset under the DUPLEX setup. These results, consistent with those in Table~\ref{tb:duplex}, highlight two key observations: (1) MLP outperforms DUPLEX on several tasks, and (2) label leakage in DUPLEX significantly impacts the results.
Additionally, Figure~\ref{fig:duplex_cls_citeseer} illustrates the number of samples and the accuracy for each class in the DUPLEX setup on the CiteSeer dataset for the 4C task. These findings, consistent with those in Figure~\ref{fig:imbalance}, further emphasize the class imbalance issue in the 4C task.
