# Supplementary material for: Rethinking Link Prediction for Directed Graphs
Source: arXiv:2502.05724 source file (2025-05-21)
Supplement: Supplementary file 4 [file appendix_proof.tex]

\hypertarget{app:proof}{} 
\section{Proof}\label{app_proof}

\hypertarget{app_proof_th_dual}{} 
\subsection{The proof of Theorem~\ref{th_dual}}\label{app_proof_th_dual}

\textbf{Theorem~\ref{th_dual}.}
For the framework defined by Equations (\ref{eq_encoder}) and (\ref{eq_decoder}), if ${d_{\theta}}, {d_{\phi}} > 0$ and sufficiently large, there exist embeddings ${\bm \theta}_u, {\bm \phi}_u$ and a decoder $\mathrm{Dec}(\cdot)$ that can correctly compute the probability $p(u,v)$ of any directed edge $(u,v)$ in an arbitrary graph. Conversely, if ${d_{\theta}} = 0$ or ${d_{\phi}} = 0$, no such embeddings or decoders can compute the correct probability of any edges in an arbitrary graph.
\begin{proof}
If ${d_{\theta}}, {d_{\phi}} > 0$ and are sufficiently large, there exist two real-valued embeddings, ${\bm \theta}_u$ and ${\bm \phi}_u$, for each node \( u \) in the graph. According to the unified framework for directed link prediction methods, these embeddings, ${\bm \theta}_u$ and ${\bm \phi}_u$, can represent the outputs of various encoder methods, including source-target methods, complex-valued methods, and gravity-inspired methods. For these encoder methods, a decoder exists that can compute the probability \( p(u, v) \) for any directed edge \( (u, v) \).
As an example, consider source-target methods. If we have two embeddings, \( \vs_u \) and \( \vt_u \), for each node \( u \), we can correctly compute the probability \( p(u, v) \) of any edge \( (u, v) \) using the expression \( p(u, v) = \sigma(\vs_u^{\top} \vt_v) \), when \( \mA_{uv} = \vs_u^{\top} \vt_v \). Based on existing embedding methods such as STRAP and HOPE~\cite{strap,hope}, it is known that there exist embeddings \( \vs_u \) and \( \vt_v \) that satisfy \( \mA_{uv} = \vs_u^{\top} \vt_v \).
For complex-valued methods, such as DUPLEX~\cite{duplex}, it has been demonstrated that there exist embeddings \( \vz_u \) and \( \vz_v \) such that \( \mH_{uv} = \vz_u \overline{\vz}_v \), where \( \overline{\vz}_v \) is the complex conjugate of \( \vz_v \).
Therefore, we conclude that there exist embeddings \( {\bm \theta}_u \) and \( {\bm \phi}_u \), along with a decoder \( \mathrm{Dec}(\cdot) \), that can correctly compute the probability \( p(u, v) \) for any directed edge \( (u, v) \) in an arbitrary graph.

If ${d_{\theta}} = 0$ or ${d_{\phi}} = 0$, this implies that each node $u$ in the graph is represented by a single real-valued embedding $\vh_u$. According to existing methods~\cite{magnet,dpyg}, there are three main types of decoders for single real-valued embeddings: 
$\sigma(\vh_u^{\top}\vh_v)$, $\mathrm{MLP}(\vh_u \odot \vh_v)$, and $\mathrm{MLP}(\vh_u \| \vh_v)$.
For the decoders $\sigma(\vh_u^{\top}\vh_v)$ and $\mathrm{MLP}(\vh_u \odot \vh_v)$, it is known that they cannot distinguish between $p(u,v)$ and $p(v,u)$. This is because 
$ \vh_v^{\top}\vh_u = \vh_u^{\top}\vh_v$ and $\vh_u \odot \vh_v = \vh_v \odot \vh_u$,
which leads to $p(u,v) = p(v,u)$. As a result, these decoders fail to compute the correct probabilities for directed edges.

Next, we demonstrate that the decoder $\mathrm{MLP}(\vh_u \| \vh_v)$ also fails to compute the probability $p(u,v)$ for certain graphs. Consider the directed ring graph (a) in Figure~\ref{fig:bg}, which consists of three nodes and three edges ($1 \to 2, 2 \to 3, 3 \to 1$). Each node is assigned a real-valued embedding, i.e., $\vh_1, \vh_2, \vh_3$. Let the decoder be a simple MLP with $\sigma = \mathrm{Sigmoid}(\cdot)$ as the activation function. For edge $1 \to 2$, the probability is given by:
\begin{equation}
    p(1,2) = \sigma(\vh_1\vw_1 + \vh_2\vw_2) > 0.5, \quad p(2,1) = \sigma(\vh_2\vw_1 + \vh_1\vw_2) < 0.5.
\end{equation}
Here, $\vw_1, \vw_2 \in \mathbb{R}^{d \times 1}$ are the learnable weights, and $d$ is the dimensionality of $\vh$. From these inequalities, we have:
\begin{equation}
    \vh_1\vw_1 + \vh_2\vw_2 > 0, \quad \vh_2\vw_1 + \vh_1\vw_2 < 0.
\end{equation}
Subtracting the second inequality from the first gives:
\begin{equation}\label{eq_1_2}
    (\vh_1 - \vh_2)\vw_1 + (\vh_2 - \vh_1)\vw_2 > 0.
\end{equation}

Similarly, for edges $2 \to 3$ and $3 \to 1$, we derive:
\begin{equation}
    (\vh_2 - \vh_3)\vw_1 + (\vh_3 - \vh_2)\vw_2 > 0, \quad (\vh_3 - \vh_1)\vw_1 + (\vh_1 - \vh_3)\vw_2 > 0.
\end{equation}

Adding these three inequalities, including Eq.~(\ref{eq_1_2}), results in $0 > 0$, which is a contradiction. Therefore, no embeddings $\vh$ and weights $\vw$ exist that can satisfy this condition. The same result holds even if nonlinearities are added to the MLP. This example demonstrates that the decoder $\mathrm{MLP}(\vh_u \| \vh_v)$ also fails to compute the probabilities for directed edges in an arbitrary graph. Hence, for existing methods, if $d_{\theta} = 0$ or $d_{\phi} = 0$, no embeddings or decoders can correctly compute the probabilities for any edges in an arbitrary graph.

\end{proof}

\hypertarget{app_proof_cora_de}{}
\subsection{The proof of Corollary~\ref{coro_de}} \label{app_proof_cora_de}

\textbf{Corollary~\ref{coro_de}.} With dual embeddings $\bm{\theta}_u$ and $\bm{\phi}_u$, if there is no suitable decoder $\mathrm{Dec(\cdot)}$, the probability $p(u,v)$ of any edge $(u,v)$ cannot be computed correctly. In contrast, even with one single embedding ($\bm{\theta}_u$ or $\bm{\phi}_u = \varnothing$), a suitable decoder can improve the ability to compute edge probabilities.
\begin{proof} 

Theorem~\ref{th_dual} establishes that dual embeddings \((\bm{\theta}_u, \bm{\phi}_u)\) combined with a suitable decoder \(\mathrm{Dec}(\cdot)\), guarantee the correct computation of \(p(u,v)\). However, if the decoder is unsuitable (e.g., it fails to model directional relationships), even valid embeddings cannot produce correct edge probabilities. For example, a symmetric decoder like \(\mathrm{Dec}(\bm{\theta}_u, \bm{\phi}_u, \bm{\theta}_v, \bm{\phi}_v) = \sigma(\bm{\theta}_u^\top \bm{\theta}_v + \bm{\phi}_u^\top \bm{\phi}_v)\) leads to \(p(u,v) = p(v,u)\), which violates directionality. This highlights that the decoder must align with the embeddings' structure to exploit their expressivity fully.

In contrast, Theorem~\ref{th_dual} shows that single embeddings (\(d_\theta = 0\) or \(d_\phi = 0\)) cannot universally represent arbitrary directed graphs. Nevertheless, a suitable decoder can still improve edge probability estimation in constrained scenarios. For example, an asymmetric decoder like \(\mathrm{Dec}(\bm{h}_u, \bm{h}_v) = \mathrm{MLP}(\bm{h}_u \| \bm{h}_v)\) can preserve some directionality by learning from the data. While such decoders fail on more complex structures like ring graphs (as shown in Theorem~\ref{th_dual}), they can handle simpler directed graph structures. In summary, dual embeddings require suitable decoders to achieve theoretical expressivity, while single embeddings, though fundamentally limited, can still benefit from specific decoders in practice.
\end{proof}

\hypertarget{app_proof_lemma_digae_conv}{}
\subsection{The proof of Lemma~\ref{lemma_digae_conv}}\label{app_proof_lemma_digae_conv}
\textbf{Lemma~\ref{lemma_digae_conv}.} When omitting degree-based normalization in Equations (\ref{digae_s}) and (\ref{digae_t}), the graph convolution of DiGAE is
\begin{equation*}
\left[\mS^{(\ell+1)},\mT^{(\ell+1)}\right]^{\top} =\sigma\left(\mathcal{S}(\hat{\mA})\left[\mS^{(\ell)}\mW_{S}^{(\ell)},\mT^{(\ell)}\mW_{T}^{(\ell)}\right]^{\top} \right). 
\end{equation*}

\begin{proof}
Substituting the block matrix $\mathcal{S}(\hat{\mA})=
    \left[ 
        \begin{array}{cc}
            \mathbf{0} & \hat{\mA} \\
            \hat{\mA}^{\top} & \mathbf{0}
        \end{array}
    \right]$ into the above convolution equation, we obtain: 
\begin{equation}
    \left[ 
        \begin{array}{c}
\mS^{(\ell+1)}\\
\mT^{(\ell+1)}
        \end{array}
    \right]=
    \sigma\left(\left[ 
        \begin{array}{cc}
            \mathbf{0} & \hat{\mA} \\
            \hat{\mA}^{\top} & \mathbf{0}
        \end{array}
    \right] 
    \left[ 
        \begin{array}{c}
\mS^{(\ell)}\mW_{S}^{(\ell)}\\
\mT^{(\ell)}\mW_{T}^{(\ell)}
        \end{array}
    \right]\right)
    = \left[ 
        \begin{array}{c}
\sigma\left(\hat{\mA}\mT^{(\ell)}\mW_{T}^{(\ell)}\right)\\
\sigma\left(\hat{\mA}^{\top}\mS^{(\ell)}\mW_{S}^{(\ell)}\right)
        \end{array}
    \right].
\end{equation}
This result corresponds exactly to Equations (\ref{digae_s}) and (\ref{digae_t}) when the degree-based normalization of $\hat{\mA}$ is not considered. If we include the normalization, it actually applies to $\mathcal{S}(\hat{\mA})$. Notably, the diagonal degree matrix of $\mathcal{S}(\hat{\mA})$ is given by $\mathrm{diag}\left(\hat{\mD}_{\rm out}, \hat{\mD}_{\rm in}\right)$. Therefore, we have:
\begin{align}
        \left[ 
        \begin{array}{c}
\mS^{(\ell+1)}\\
\mT^{(\ell+1)}
        \end{array}
    \right]&=
    \sigma\left(
    \left[ 
        \begin{array}{cc}
            \hat{\mD}_{\rm out}^{-\beta} &\mathbf{0} \\
            \mathbf{0} & \hat{\mD}_{\rm in}^{-\alpha}
        \end{array}
    \right]
    \left[ 
        \begin{array}{cc}
            \mathbf{0} & \hat{\mA} \\
            \hat{\mA}^{\top} & \mathbf{0}
        \end{array}
    \right] 
    \left[ 
        \begin{array}{cc}
             \hat{\mD}_{\rm out}^{-\beta} &\mathbf{0} \\
            \mathbf{0} & \hat{\mD}_{\rm in}^{-\alpha}
        \end{array}
    \right]
    \left[ 
        \begin{array}{c}
\mS^{(\ell)}\mW_{S}^{(\ell)}\\
\mT^{(\ell)}\mW_{T}^{(\ell)}
        \end{array}
    \right]\right) \\
    &= \left[ 
        \begin{array}{c}
\sigma\left(\hat{\mD}_{\rm out}^{-\beta}\hat{\mA}\hat{\mD}_{\rm in}^{-\alpha}\mT^{(\ell)}\mW_{T}^{(\ell)}\right)\\
\sigma\left(\hat{\mD}_{\rm in}^{-\alpha}\hat{\mA}^{\top}\hat{\mD}_{\rm out}^{-\beta}\mS^{(\ell)}\mW_{S}^{(\ell)}\right)
        \end{array}
    \right].
\end{align}
This result aligns exactly with the graph convolution of DiGAE in Equations (\ref{digae_s}) and (\ref{digae_t}).
\end{proof}

%\begin{align}
%\mS^{(\ell+1)} &= \sigma\left((\hat{\mD}_{\rm out})^{-\beta}\hat{\mA}(\hat{\mD}_{\rm in})^{-\alpha}\mT^{(\ell)}\mW_{T}^{(\ell)}\right), \label{digae_s}\\
%\mT^{(\ell+1)} &= \sigma\left((\hat{\mD}_{\rm in})^{-\alpha}\hat{\mA}^{\top}(\hat{\mD}_{\rm out})^{-\beta}\mS^{(\ell)}\mW_{S}^{(\ell)}\right),\label{digae_t}
%\end{align}

\hypertarget{app_proof_le_norm}{}
\subsection{The proof of Lemma~\ref{le:norm}}\label{app_proof_le_norm}
\textbf{Lemma~\ref{le:norm}.} The symmetrically normalized block adjacency matrix $ \mD_{\mathcal{S}}^{-1/2} \mathcal{S}(\hat{\mA}) \mD_{\mathcal{S}}^{-1/2}=\mathcal{S}(\Tilde{\mA}) $, where $\mD_{\mathcal{S}} = \mathrm{diag}(\hat{\mD}_{\rm out}, \hat{\mD}_{\rm in})$ is the diagonal degree matrix of \(\mathcal{S}(\hat{\mA})\).
\begin{proof}
     For the block adjacency matrix $\mathcal{S}(\hat{\mA})=
    \left[\begin{array}{cc}
        \mathbf{0} & \hat{\mA}\\
        \hat{\mA}^{\top} & \mathbf{0}
    \end{array} \right]$ and its degree matrix $\mD_{\mathcal{S}}= \left[\begin{array}{cc}
        \hat{\mD}_{\rm out} & \mathbf{0}\\
        \mathbf{0} & \hat{\mD}_{\rm in}
    \end{array} \right]$, we have 
    \begin{align}
    \mD_{\mathcal{S}}^{-1/2}\mathcal{S}(\hat{\mA})\mD_{\mathcal{S}}^{-1/2} 
    &=
    \left[\begin{array}{cc}
        \hat{\mD}_{\rm out} & \mathbf{0}\\
        \mathbf{0} & \hat{\mD}_{\rm in}
    \end{array} \right]^{-1/2}
    \left[\begin{array}{cc}
        \mathbf{0} & \hat{\mA}\\
        \hat{\mA}^{\top} & \mathbf{0}
    \end{array} \right]
    \left[\begin{array}{cc}
        \hat{\mD}_{\rm out} & \mathbf{0}\\
        \mathbf{0} & \hat{\mD}_{\rm in}
    \end{array} \right]^{-1/2}\\
    &=
    \left[\begin{array}{cc}
        \hat{\mD}_{\rm out}^{-1/2} & \mathbf{0}\\
        \mathbf{0} & \hat{\mD}_{\rm in}^{-1/2}
    \end{array} \right]
    \left[\begin{array}{cc}
        \mathbf{0} & \hat{\mA}\\
        \hat{\mA}^{\top} & \mathbf{0}
    \end{array} \right]
    \left[\begin{array}{cc}
        \hat{\mD}_{\rm out}^{-1/2} & \mathbf{0}\\
        \mathbf{0} & \hat{\mD}_{\rm in}^{-1/2}
    \end{array} \right]\\
    &=
    \left[\begin{array}{cc}
        \mathbf{0} & \hat{\mD}_{\rm out}^{-1/2}\hat{\mA}\hat{\mD}_{\rm in}^{-1/2}\\
        \left(\hat{\mD}_{\rm out}^{-1/2}\hat{\mA}\hat{\mD}_{\rm in}^{-1/2} \right)^{\top} & \mathbf{0}
    \end{array} \right]\\
    &=
     \left[\begin{array}{cc}
        \mathbf{0} & \Tilde{\mA}\\
        \Tilde{\mA^{\top}} & \mathbf{0}
    \end{array} \right]\\
    &=
    \mathcal{S}(\Tilde{\mA}).
    \end{align}
\end{proof}
