# Supplementary material for: Rethinking Link Prediction for Directed Graphs
Source: arXiv:2502.05724 source file (2025-05-21)
Supplement: Supplementary file 5 [file appendix_sdgae.tex]

\hypertarget{app_sdgae}{} 
\section{Details and Experimental Setting for SDGAE}\label{app_sdgae}

\hypertarget{app_sdgae_conv}{} 
\subsection{More details of graph convolution}\label{app_sdgae_conv}
The graph convolutional layer of SDGAE is defined as: 
\begin{equation}\label{eq:app_bg_A_hat}
    \left[ 
        \begin{array}{c}
            \mS^{(\ell+1)} \\
            \mT^{(\ell+1)}
        \end{array}
    \right] =
    \left[ 
        \begin{array}{c}
            w^{(\ell)}_S \\
            w^{(\ell)}_T
        \end{array}
    \right] 
    \odot
    \left[ 
        \begin{array}{cc}
            \mathbf{0} & \Tilde{\mA} \\
            \Tilde{\mA}^{\top} & \mathbf{0}
        \end{array}
    \right]
    \left[ 
        \begin{array}{c}
            \mS^{(\ell)} \\
            \mT^{(\ell)}
        \end{array}
    \right] 
    +
    \left[ 
        \begin{array}{c}
            \mS^{(\ell)} \\
            \mT^{(\ell)}
        \end{array}
    \right].
\end{equation}
Expanding this formulation, the source and target embeddings at each layer are denoted as:
\begin{equation}\label{app_eq_sdgae}
    \mS^{(\ell+1)} =w_{S}^{(\ell)}\Tilde{\mA}\mT^{(\ell)}+\mS^{(\ell)}, \quad \mT^{(\ell+1)} =w_{T}^{(\ell)}\Tilde{\mA}^{\top}\mS^{(\ell)}+\mT^{(\ell)}.
\end{equation}
If we denote $\mX_S = \mS^{(0)}=\mathrm{MLP}_S(\mX)$ and $\mX_T = \mT^{(0)}=\mathrm{MLP}_T(\mX)$, we can derive:
\begin{align*}
\mS^{(1)} &= w_{S}^{(0)}\Tilde{\mA}\mX_T + \mX_S, \\
\mT^{(1)} &= w_{T}^{(0)}\Tilde{\mA}^{\top}\mX_S + \mX_T, \\
\mS^{(2)} &= \mX_S + \left(w_{S}^{(1)} + w_{S}^{(0)}\right)\Tilde{\mA}\mX_T + w_{S}^{(1)}w_{T}^{(0)}\Tilde{\mA}\Tilde{\mA}^{\top}\mX_S, \\
\mT^{(2)} &= \mX_T + \left(w_{T}^{(1)} + w_{T}^{(0)}\right)\Tilde{\mA}^{\top}\mX_S + w_{T}^{(1)}w_{S}^{(0)}\Tilde{\mA}^{\top}\Tilde{\mA}\mX_T.
\end{align*}
%The result shows the source and target embeddings corresponding to the number of layers $L=1$ and $L=2$. It can be found that the propagation is very similar to the spectral-based GNNs. Specifically, the propagation expression of the spectral-based GNNs is $\mY = \nolimits\sum_{\ell=0}^{L}w_{\ell}\Tilde{\mA}^{\ell}$, where $w_{\ell}$ denotes the learnable polynomial weights and $\Tilde{\mA}$ denotes the symmetrically normalised undirected graph adjacency matrix. By comparison, it can be found that SDGAE also achieves spectral--based propagation by learning different weights $w_S$ and $w_T$, and further spectrum analyses about it will be the subject of further research.
These results represent the source and target embeddings for layers \(L=1, 2\). The propagation pattern closely resembles that of spectral-based GNNs~\cite{gprgnn,bernnet,chebnetii}. Specifically, the propagation in spectral-based GNNs is expressed as \(\mY = \sum_{\ell=0}^{L}w_{\ell}\Tilde{\mA}^{\ell}\), where \(w_{\ell}\) denotes the learnable polynomial weights and \(\Tilde{\mA}\) represents the symmetrically normalized adjacency matrix of an undirected graph. By comparison, SDGAE achieves spectral-based propagation by learning separate weights \(w_S\) and \(w_T\). Further spectrum analysis of SDGAE will be explored in future research.

\textbf{Time Complexity}. The primary time complexity of SDGAE arises from the graph convolution process. Based on Equation~(\ref{app_eq_sdgae}), the time complexity of SDGAE's convolution is given by \( O(2Lmd) \), where \( m \) is the number of edges, \( L \) is the number of layers, and \( d \) is the embedding dimension. This complexity scales linearly with \( m \) and is lower than that of DiGAE, which involves multiple learnable weight matrices.

\begin{wraptable}{r}{105mm}
\centering
\vspace{-8mm}
\caption{The parameters of SDGAE on different datasets.}
\begin{tabular}{lcccccc}
\toprule
Datasets &hidden &embedding &MLP layer &$L$ &lr &wd  \\ \midrule
Cora-ML & 64 & 64 &1 &5 &0.01 &0.0 \\
CiteSeer& 64 & 64 &1 &5 &0.01 &0.0 \\
Photo & 64 & 64 &2 &5 &0.005 &0.0 \\
Computers & 64 & 64 &2 & 3 & 0.005 &0.0\\
WikiCS & 64 & 64 & 2&5 & 0.005 &5e-4 \\
Slashdot & 64 & 64 &2 &5 &0.01 & 5e-4 \\
Epinions & 64 & 64 &2 &5 & 0.005 &0.0 \\
\bottomrule
\end{tabular}
\vspace{-2mm}
\label{app_para_sdage}
\end{wraptable}

\hypertarget{app_sdgae_setting}{} 
\subsection{Experimental setting}\label{app_sdgae_setting}
For the SDGAE experimental setting, we aligned our settings with those of other baselines in DirLinkBench to ensure fairness. For the MLP used in $\mX$ initialization, we set the number of layers to one or two, matching DiGAE's convolutional layer configurations. The number of hidden units and the embedding dimension were both set to 64. The learning rate (lr) was chosen as either 0.01 or 0.005, and weight decay (wd) was set to 0.0 or 5e-4, following the configurations of most GNN baselines. The number of convolutional layers $L$ was set to 3, 4, or 5. We performed a grid search to optimize parameters on the validation set, and Table~\ref{app_para_sdage} presents the corresponding SDGAE parameters for different datasets.
